# Supplementary material for: Effective Elastic Wave Characteristics of Composite Media
Source: arXiv:2012.15214 ancillary file (2020-12-30)
Supplement: Supplementary file 1 [file SM.pdf]

# Supplementary Material - Effective Elastic Wave Characteristics of Composite Media

Jaeuk Kim[1] and Salvatore Torquato[1,2,3,4,*]
[1] Department of Physics, Princeton University, Princeton, New Jersey 08544, USA
[2] Department of Chemistry, Princeton University, Princeton, New Jersey 08544, USA
[3] Princeton Institute for the Science and Technology of Materials, Princeton University, Princeton, New Jersey 08544, USA
[4] Program in Applied and Computational Mathematics, Princeton University, Princeton, New Jersey 08544, USA
[*] torquato@princeton.edu

## I. DERIVATION OF LOCAL STRONG-CONTRAST EXPANSIONS

Here we present a detailed derivation of the local strong-contrast expansion presented in the main text. Aforementioned, we consider a macroscopically large ellipsoidal two-phase composite specimen in $\mathbb{R}^d$ embedded inside an infinitely large reference phase of mass density $\rho_I$ and stiffness tensor $\boldsymbol{C}_I$. We assume that the microstructure is perfectly general, and the inhomogeneity length scales $\ell$ are much smaller than the size of specimen $L$, i.e., $\ell \ll L$. The shape of this specimen is purposely chosen to be non-spherical since any rigorously correct expression for the effective stiffness tensor must ultimately be independent of the shape of the composite specimen in the infinite-volume limit. The local stiffness tensor $\boldsymbol{C}(\mathbf{x})$ and mass density $\rho(\mathbf{x})$ of a two-phase composite are written respectively as

$$\boldsymbol{C}(\mathbf{x}) \equiv \boldsymbol{C}_1 \mathcal{I}^{(1)}(\mathbf{x}) + \boldsymbol{C}_2 \mathcal{I}^{(2)}(\mathbf{x}), \tag{S1}$$

$$\rho(\mathbf{x}) \equiv \rho_1 \mathcal{I}^{(1)}(\mathbf{x}) + \rho_2 \mathcal{I}^{(2)}(\mathbf{x}), \tag{S2}$$

where for phase $i$ $(=1,2)$, $\boldsymbol{C}_i$ is the stiffness tensor, $\rho_i$ is the mass density, and $\mathcal{I}^{(i)}(\mathbf{x})$ is the phase indicator (see Sec. II in the main text). Now suppose the incident plane strain waves $\boldsymbol{\epsilon}_0(\mathbf{x})$ of an angular frequency $\omega$ and wavevector $\mathbf{k}_I(\omega)$ in the reference phase, i.e.,

$$\boldsymbol{\epsilon}_0(\mathbf{x}) = \tilde{\boldsymbol{\epsilon}}_0 \exp(i(\mathbf{k}_I(\omega)\cdot\mathbf{x} - \omega t)). \tag{S3}$$

The associated wavelengths $\lambda = 2\pi/|\mathbf{k}_I|$ must lie between the inhomogeneity length scales $\ell$ and the specimen size $L$ [1]. Granting that the effective-medium description is valid for the composite, we obtain the corresponding stiffness tensor $\boldsymbol{C}_e(\mathbf{k}_I, \omega)$.

In the ensuing derivation, we take the reference phase to be phase $q$ $(=1,2)$ and make the following five assumptions, in which three are associated with phase properties, one is related to wavelengths, and the last assumes Hooke's law:

(a) Phase 1 and phase 2 are elastically isotropic, i.e.,

$$\boldsymbol{C}_i = dK_i\,\boldsymbol{\Lambda}_h + 2G_i\,\boldsymbol{\Lambda}_s, \quad (i=1,2) \tag{S4}$$

where $K_i$ and $G_i$ are bulk and shear moduli of phase $i$ $(=1,2)$, respectively. Here, the *hydrostatic projection tensor* $\boldsymbol{\Lambda}_h$ and *shear projection tensor* $\boldsymbol{\Lambda}_s$ are constant fourth-rank tensors (defined in the main text).

(b) Each phase is dissipationless, namely, the elastic moduli $K_i$ and $G_i$ for $i=1,2$ are real-valued and frequency-independent.

(c) The mass densities of both phases are identical, i.e.,

$$\rho_1 = \rho_2 = \rho_e. \tag{S5}$$

(d) The long-wavelength (qausistatic) regime is assumed, i.e., $\lambda \gg \ell$.

(e) We assume infinitesimal deformations, implying the *Hooke's law*.

Implications of assumptions (a)-(c) are discussed in Sec. II in the main text. Among them, we only state here that assumptions (a) and (b) imply the linear dispersion relation in the reference phase [i.e., $k_{L_q}(\omega) = \omega/c_{L_q}$ and $k_{T_q}(\omega) = \omega/c_{T_q}$ for longitudinal and transverse waves, respectively]. Henceforth we replace the argument $\omega$ in functions with $k_{L_q}$ and do not explicitly indicate the $\omega$ dependence.

We derive some important integral equations for local fields in Sec. I A. We then derive the local strong-contrast expansions for a macroscopically anisotropic medium in Sec. I B. In Sec. I C, we then simplify the expansions derived in Sec. I B by assuming the composite is macroscopically isotropic.

### A. Integral Equations for the Cavity Strain Field

Here we first derive general expressions for an anisotropic reference phase $q$ and then simplify the results by assuming (a). Due to assumption (e), we can use the Hooke's law to relate the local stress $\boldsymbol{\tau}(\mathbf{x})$ to the local strain $\boldsymbol{\epsilon}(\mathbf{x})$

$$\boldsymbol{\tau}(\mathbf{x}) = \boldsymbol{C}(\mathbf{x}) : \boldsymbol{\epsilon}(\mathbf{x}), \tag{S6}$$

where $\boldsymbol{C}(\mathbf{x})$ is given in (S1), and the strain tensor is the symmetric part of the gradient of displacement field $\mathbf{u}(\mathbf{x})$, i.e.,

$$\boldsymbol{\epsilon}(\mathbf{x}) \equiv \frac{1}{2}\Big[\boldsymbol{\nabla}\mathbf{u} + (\boldsymbol{\nabla}\mathbf{u})^T\Big]. \tag{S7}$$

Using separation of variables $\boldsymbol{u}(\mathbf{x}, t) \to \boldsymbol{u}(\mathbf{x})\, e^{-i\omega t}$, one can write the time-harmonic equation of motion of the volume element at $\mathbf{x}$ as

$$-\omega^2 \rho(\mathbf{x})\, \boldsymbol{u}(\mathbf{x}) = \boldsymbol{\nabla} \cdot \boldsymbol{\tau}(\mathbf{x}). \tag{S8}$$

We now introduce the *induced stress polarization field* defined by

$$\boldsymbol{P}(\mathbf{x}) \equiv \left(\frac{\boldsymbol{C}(\mathbf{x})}{\rho(\mathbf{x})} - \frac{\boldsymbol{C}_q}{\rho_q}\right) : \boldsymbol{\epsilon}(\mathbf{x}), \tag{S9}$$

which is a symmetric, second-rank tensor that is non-zero only in the "polarized" phase $p(\neq q)$. Using Eqs. (S8) and (S9), we obtain an inhomogeneous elastic wave equation in the reference phase whose source term arises from the inhomogeneity of the stiffness and mass density. This wave equation is written in component form as

$$\omega^2\, \check{u}_i(\mathbf{x}) + \frac{(C_q)_{ijkl}}{\rho_q} \frac{\partial^2\, \check{u}_l(\mathbf{x})}{\partial x_j \partial x_k} = -\frac{\partial P_{ij}}{\partial x_j} + \frac{\partial}{\partial x_j}\left[\frac{1}{\rho(\mathbf{x})}\right] C_{ijkl}(\mathbf{x})\, \epsilon_{kl}, \qquad \check{u}_i(\mathbf{x}) \to 0 \quad \text{as } |\mathbf{x}| \to \infty, \tag{S10}$$

where $\check{\boldsymbol{u}}(\mathbf{x}) \equiv \boldsymbol{u}(\mathbf{x}) - \boldsymbol{u_0}(\mathbf{x})$ is the displacement field in excess of the displacement field applied at infinity $\boldsymbol{u_0}(\mathbf{x})$. Importantly, comparing with the static counterpart [2, 3], Eq. (S10) has an extra term $\boldsymbol{\nabla}\Big[\rho(\mathbf{x})^{-1}\Big] \cdot \boldsymbol{\tau}(\mathbf{x})$ on the right-hand side which represents the force per area on the interface between phases $p$ and $q$ due to the internal stress. In this work, we have removed this term by assuming (c) because this simplification makes the dynamic problem formally identical to the static strong-contrast expansions studied in Refs. [2, 3]. Thus, we follow the static strong-contrast expansion formalism closely in the ensuing derivation.

Using the Green function formalism, the excessive displacement field $\check{u}_i(\mathbf{x})$ can be expressed as

$$\check{u}_i(\mathbf{x}) = \int d\mathbf{x}'\, g_{ij}^{(q)}(\mathbf{x}, \mathbf{x}') \left[\frac{\partial\, P_{jk}(\mathbf{x}')}{\partial x'_k}\right], \tag{S11}$$

where $g_{ij}^{(q)}(\mathbf{x}, \mathbf{x}')$ is the infinite-space Green's function of elastic wave equation with respect to the reference phase $q$ that satisfies

$$\omega^2\, g_{km}^{(q)}(\mathbf{x}, \mathbf{x}') + \frac{(C_q)_{ijkl}}{\rho_q} \frac{\partial^2\, g_{im}^{(q)}(\mathbf{x}, \mathbf{x}')}{\partial x_j \partial x_k} = -\delta_{km}\, \delta(\mathbf{x} - \mathbf{x}'), \qquad g_{ij}^{(q)}(\mathbf{x}, \mathbf{x}') \to 0, \quad |\mathbf{x} - \mathbf{x}'| \to \infty, \tag{S12}$$

where we that $g_{ij}^{(q)}(\mathbf{x}, \mathbf{x}') = g_{ij}^{(q)}(\mathbf{x} - \mathbf{x}')$.

To obtain an expression for strain tensor, we take the symmetric part of the gradient of Eq (S11) given as (see Sec. II for details)

$$\epsilon_{ij}(\mathbf{x}) - (\epsilon_0)_{ij}(\mathbf{x}) = \int G_{ijkl}^{(q)}(\mathbf{x} - \mathbf{x}')\, P_{kl}(\mathbf{x}')\, d\mathbf{x}', \tag{S13}$$

$$= \underbrace{-\, D_{ijkl}^{(q)}\, P_{kl}(\mathbf{x})}_{\text{inside the exclusion-region}} + \underbrace{\int_\epsilon H_{ijkl}^{(q)}(\mathbf{x} - \mathbf{x}')\, P_{kl}(\mathbf{x}')\, \mathrm{d}\mathbf{x}'}_{\text{outside the exclusion-region}}, \tag{S14}$$

where we note that, due to the singular nature of Green's function around the origin (i.e., $\mathbf{x}-\mathbf{x}'=\mathbf{0}$), the integral (S13) should be separated into two parts; one is the integral inside an infinitesimal exclusion region around the origin, and another is the integral outside the exclusion region (denoted by $\int_\epsilon \mathrm{d}\mathbf{x}'$). Thus, the fourth-rank Green's function can be written concisely as

$$\boldsymbol{G}^{(q)}(\mathbf{x},\mathbf{x}') = -\boldsymbol{D}^{(q)}\,\delta(\mathbf{x}-\mathbf{x}') + \boldsymbol{H}^{(q)}(\mathbf{x}-\mathbf{x}'), \tag{S15}$$

where the fourth-rank constant tensor $\boldsymbol{D}^{(q)}$ depends on the shape of exclusion region. The fourth-rank tensor field $H^{(q)}_{ijkl}(\mathbf{r})$ is associated with the double gradient of the dyadic Green function $g^{(q)}_{ij}(\mathbf{r})$ [cf. (S12)] given as

$$H^{(q)}_{ijkl}(\mathbf{r}) \equiv \frac{1}{4}\left[\frac{\partial^2 g^{(q)}_{ik}}{\partial x_j \partial x_l} + \frac{\partial^2 g^{(q)}_{jk}}{\partial x_i \partial x_l} + \frac{\partial^2 g^{(q)}_{il}}{\partial x_j \partial x_k} + \frac{\partial^2 g^{(q)}_{jl}}{\partial x_i \partial x_k}\right], \tag{S16}$$

which is symmetric under the following index exchanges, i.e.,

$$H^{(q)}_{ijkl}(\mathbf{r}) = H^{(q)}_{jikl}(\mathbf{r}) = H^{(q)}_{ijlk}(\mathbf{r}) = H^{(q)}_{klij}(\mathbf{r}). \tag{S17}$$

Excluding the contribution from a exclusion-region in Eq. (S14), we obtain an integral equation for the *cavity strain* tensor $\boldsymbol{f}(\mathbf{x})$ given as

$$\begin{aligned}\boldsymbol{f}(\mathbf{x}) &\equiv \boldsymbol{\epsilon}(\mathbf{x}) + \boldsymbol{D}^{(q)} : \boldsymbol{P}(\mathbf{x}) && \text{(S18)}\\ &= \boldsymbol{\epsilon}_0(\mathbf{x}) + \int_\epsilon d\mathbf{x}'\, \boldsymbol{H}^{(q)}(\mathbf{x}-\mathbf{x}') : \boldsymbol{P}(\mathbf{x}') && \text{(S19)}\\ &= \left\{\boldsymbol{I} + \boldsymbol{D}^{(q)} : [\boldsymbol{C}(\mathbf{x}) - \boldsymbol{C}_q]/\rho_e\right\} : \boldsymbol{\epsilon}(\mathbf{x}), && \text{(S20)}\end{aligned}$$

where the relation (S20) is obtained from (S18) and (S9). The cavity strain field is the elasticity analog of the Lorentz electric field used in the static strong-contrast expansion for the effective dielectric tensor [4, 5].

Eliminating $\boldsymbol{\epsilon}_0$ in Eqs. (S20) and (S9) yields the following relation:

$$\boldsymbol{P}(\mathbf{x}) = \boldsymbol{\mathcal{L}}^{(q)}(\mathbf{x}) : \boldsymbol{f}(\mathbf{x}), \tag{S21}$$

where the fourth-order tensor $\boldsymbol{\mathcal{L}}^{(q)}(\mathbf{x})$ is a linear fractional transformation of $\boldsymbol{C}(\mathbf{x})$ given by

$$\begin{aligned}\boldsymbol{\mathcal{L}}^{(q)}(\mathbf{x}) &\equiv [\boldsymbol{C}(\mathbf{x}) - \boldsymbol{C}_q]/\rho_q : \left\{\boldsymbol{I} + \boldsymbol{D}^{(q)} : [\boldsymbol{C}(\mathbf{x}) - \boldsymbol{C}_q]/\rho_q\right\}^{-1} && \text{(S22)}\\ &= \boldsymbol{L}^{(q)}\,\mathcal{I}^{(p)}(\mathbf{x}), && \text{(S23)}\end{aligned}$$

where $\boldsymbol{L}^{(q)} \equiv (\boldsymbol{C}_p - \boldsymbol{C}_q)/\rho_q : \left[\boldsymbol{I} + \boldsymbol{D}^{(q)} : (\boldsymbol{C}_p - \boldsymbol{C}_q)/\rho_q\right]^{-1}$. Note that $\boldsymbol{L}^{(q)}$ is identical to its static counterpart.

We now assume phase 1 and 2 are isotropic [cf. (a)] to provide explicit formulas for $\boldsymbol{g}^{(q)}(\mathbf{r})$, $\boldsymbol{H}^{(q)}(\mathbf{r})$, $\boldsymbol{D}^{(q)}$, and $\boldsymbol{L}^{(q)}$ which are used in the main text. The reader is referred to Sec. II for detail of derivations. The dyadic Green function defined in Eq. (S12) can be simplified as

$$g^{(q)}_{ij}(\mathbf{r}) = A_d(r)\,\hat{\mathbf{r}}_i\hat{\mathbf{r}}_j + B_d(r)\,\delta_{ij}, \tag{S24}$$

where $r \equiv |\mathbf{r}|$, $\hat{\mathbf{r}} \equiv \mathbf{r}/|\mathbf{r}|$, $\hat{\mathbf{r}}_i$ is the $i$th component of $\hat{\mathbf{r}}$, and $A_d(r)$ and $B_d(r)$ are given by Eqs. (S94) and (S95), respectively. For $d=3$, (S24) is simply expressed as

$$\begin{aligned}g^{(q)}_{ij}(\mathbf{r}) = \frac{1}{4\pi\omega^2 r^3}\Big(&\left\{e^{ik_{L_q}r}(1 - i\,k_{L_q} r) - e^{ik_{T_q}r}[1 - i\,k_{T_q} r - (k_{T_q} r)^2]\right\}\delta_{ij}\\ &+ \left\{e^{ik_{L_q}r}[-3 + i3\,k_{L_q} r + (k_{L_q} r)^2] + e^{ik_{T_q}r}[3 - i3\,k_{T_q} r - (k_{T_q} r)^2]\right\}\hat{\mathbf{r}}_i\hat{\mathbf{r}}_j\Big).\end{aligned} \tag{S25}$$

Use (S25) and (S16) yields an explicit expression for $\boldsymbol{H}^{(q)}$ in an isotropic phase:

$$\begin{aligned}\boldsymbol{H}^{(q)}(\mathbf{r}) =& \frac{-i\pi}{2(2\pi)^{d/2}}\frac{1}{\omega^2 r^{d+2}}\\ &\times\Big\{\left[r_L^{d/2+1}\,\mathcal{H}^{(1)}_{d/2+1}(r_L) - r_T^{d/2+1}\,\mathcal{H}^{(1)}_{d/2+1}(r_T)\right](d\,\boldsymbol{\Lambda}_h + 2\,\boldsymbol{I}) + r_T^{d/2+2}\,\mathcal{H}^{(1)}_{d/2}(r_T)\,\boldsymbol{I}\\ &\quad - \left[r_L^{d/2+2}\,\mathcal{H}^{(1)}_{d/2+2}(r_L) - r_T^{d/2+2}\,\mathcal{H}^{(1)}_{d/2+2}(r_T)\right][2\,\boldsymbol{T}_1(\mathbf{r}) + 4\,\boldsymbol{T}_2(\mathbf{r})] - r_T^{d/2+3}\,\mathcal{H}^{(1)}_{d/2+1}(r_T)\,\boldsymbol{T}_2(\mathbf{r})\\ &\quad + \left[r_L^{d/2+3}\,\mathcal{H}^{(1)}_{d/2+3}(r_L) - r_T^{d/2+3}\,\mathcal{H}^{(1)}_{d/2+3}(r_T)\right]\boldsymbol{T}_3(\mathbf{r})\Big\},\end{aligned} \tag{S26}$$

where $r_L \equiv k_{L_q} r$, $r_T \equiv k_{T_q} r$, and three fourth-rank tensors $\boldsymbol{T}_i(\mathbf{r})$ for $i = 1, 2, 3$ are defined as

$$(T_1)_{ijkl}(\mathbf{r}) \equiv \frac{1}{2}(\delta_{ij}\hat{\mathbf{r}}_k\hat{\mathbf{r}}_l + \hat{\mathbf{r}}_i\hat{\mathbf{r}}_j\delta_{kl}), \tag{S27}$$

$$(T_2)_{ijkl}(\mathbf{r}) \equiv \frac{1}{4}(\hat{\mathbf{r}}_i\,\delta_{jk}\,\hat{\mathbf{r}}_l + \hat{\mathbf{r}}_j\,\delta_{ik}\,\hat{\mathbf{r}}_l + \hat{\mathbf{r}}_i\,\delta_{jl}\,\hat{\mathbf{r}}_k + \hat{\mathbf{r}}_j\,\delta_{il}\,\hat{\mathbf{r}}_k), \tag{S28}$$

$$(T_3)_{ijkl}(\mathbf{r}) \equiv \hat{\mathbf{r}}_i\hat{\mathbf{r}}_j\hat{\mathbf{r}}_k\hat{\mathbf{r}}_l. \tag{S29}$$

Note that (S26) reduces to its static counterpart given in Refs. [2, 3, 6] up to a multiplicative factor $\rho_q$:

$$\lim_{\omega\to 0^+} \boldsymbol{H}^{(q)}(\mathbf{r}) = \frac{\Gamma(d/2)}{4\pi^{d/2}}\frac{1}{d\,{c_{L_q}}^2}\frac{1}{r^d}\Big[\alpha_q d\,\boldsymbol{\Lambda}_h - 2d\,\boldsymbol{I} - 2d\alpha_q\,\boldsymbol{T}_1(\mathbf{r}) + 2d(d-\alpha_q)\,\boldsymbol{T}_2(\mathbf{r}) + d(d+2)\alpha_q\,\boldsymbol{T}_3(\mathbf{r})\Big], \tag{S30}$$

where $\alpha_q \equiv dK_q/G_q + (d-2) = d({c_{L_q}}^2 - {c_{T_q}}^2)/{c_{T_q}}^2$. The Fourier transforms of the Green function $G^{(q)}_{ijkl}(\mathbf{r})$ and $H^{(q)}_{ijkl}(\mathbf{r})$ are simple:

$$\begin{aligned}\tilde{G}^{(q)}_{ijkl}(\mathbf{q}) = &-\frac{q^4}{\omega^2}\left(\frac{1}{q^2-{k_{L_q}}^2} - \frac{1}{q^2-{k_{T_q}}^2}\right)\hat{\mathbf{q}}_i\hat{\mathbf{q}}_j\hat{\mathbf{q}}_k\hat{\mathbf{q}}_l \\ &- \frac{1}{{c_{T_q}}^2}\frac{1}{q^2-{k_{T_q}}^2}\frac{1}{4}(\hat{\mathbf{q}}_i\,\delta_{jk}\,\hat{\mathbf{q}}_l + \hat{\mathbf{q}}_j\,\delta_{ik}\,\hat{\mathbf{q}}_l + \hat{\mathbf{q}}_i\,\delta_{jl}\,\hat{\mathbf{q}}_k + \hat{\mathbf{q}}_j\,\delta_{il}\,\hat{\mathbf{q}}_k),\end{aligned} \tag{S31}$$

and $\tilde{H}^{(q)}_{ijkl}(\mathbf{q})$ is given in Eq. (S36).

The constant tensors $\boldsymbol{D}^{(q)}$ and $\boldsymbol{L}^{(q)}$ depend on the exclusion-region shape. For a spherical exclusion-region in $\mathbb{R}^d$, $\boldsymbol{D}^{(q)}$ defined in Eq. (S14) writes explicitly as

$$\begin{aligned}\boldsymbol{D}^{(q)} &= \frac{\rho_e\,\boldsymbol{\Lambda}_h}{dK_q + 2(d-1)G_q} + \frac{\rho_e d(K_q+2G_q)\,\boldsymbol{\Lambda}_s}{G_q(d+2)[dK_q+2(d-1)G_q]} \\ &= \frac{1}{d{c_{L_q}}^2}\boldsymbol{\Lambda}_h + \frac{1}{d+2}\left(\frac{2}{d{c_{L_q}}^2} + \frac{1}{{c_{T_q}}^2}\right)\boldsymbol{\Lambda}_s\,,\end{aligned} \tag{S32}$$

where $c_{L_q}$ and $c_{T_q}$ are the longitudinal and transverse wave speeds; see the definitions in the main text. Thus, the corresponding constant tensor $\boldsymbol{L}^{(q)}$ [(S23)] is explicitly written as

$$\boldsymbol{L}^{(q)} = d{c_{L_q}}^2\left[\kappa_{pq}\boldsymbol{\Lambda}_h + \frac{(d+2){c_{T_q}}^2}{d{c_{L_q}}^2 + 2{c_{T_q}}^2}\mu_{pq}\boldsymbol{\Lambda}_s\right], \tag{S33}$$

where $\kappa_{pq}$ is the *polarizability for bulk modulus* and $\mu_{pq}$ is the *polarizability for shear modulus*, which are defined respectively as

$$\kappa_{pq} = \frac{K_p - K_q}{K_p + 2(d-1)G_q/d}, \tag{S34}$$

$$\mu_{pq} = \frac{G_p - G_q}{G_p + [dK_q/2 + (d+1)(d-2)G_q/d]\,G_q/(K_q+2G_q)}. \tag{S35}$$

**Remarks:**

1. The reference phase $q$ employed in the Green function $\boldsymbol{G}^{(q)}(\mathbf{r})$ can be different from phase 1 or 2. In this work, however, we focus on the cases where $q$ equals 1 or 2 for simplicity.
2. In rigorous sense, equation (S15) should be written as

$$\boldsymbol{G}^{(q)}(\mathbf{x},\mathbf{x}') = \begin{cases} -\boldsymbol{D}^{(q)}\,\delta(\mathbf{x}-\mathbf{x}'), & \text{outside the exclusion region,} \\ \boldsymbol{H}^{(q)}(\mathbf{x}-\mathbf{x}'), & \text{inside the exclusion region.}\end{cases}$$

Due to this definition, while $\boldsymbol{H}^{(q)}(\mathbf{r})$ in the direct-space is independent of the exclusion-region shape, the Fourier transform $\tilde{\boldsymbol{H}}^{(q)}(\mathbf{q})$ does depend on the exclusion-region shape in the following manner

$$\begin{aligned}\tilde{\boldsymbol{H}}^{(q)}(\mathbf{q}) &= \int \mathrm{d}\mathbf{r}\, e^{-i\mathbf{q}\cdot\mathbf{r}}\,\boldsymbol{H}^{(q)}(\mathbf{r}) = \int_\epsilon \mathrm{d}\mathbf{r}\, e^{-i\mathbf{q}\cdot\mathbf{r}}\,\boldsymbol{H}^{(q)}(\mathbf{r}) \\ &= \tilde{\boldsymbol{G}}^{(q)}(\mathbf{q}) + \boldsymbol{D}^{(q)}\,.\end{aligned} \tag{S36}$$

### B. Local Strong-Contrast Expansions in General Cases

Here we derive the local strong-contrast expansions for the effective stiffness tensor of a macroscopically anisotropic medium that are strictly valid in the long-wavelength (quasistatic) regime. To do so, we derive an exact series expansion for the effective tensor $\boldsymbol{L}_e^{(q)}$ in a local homogenized relation

$$\langle \boldsymbol{f}\rangle(\mathbf{x}) = \boldsymbol{L}_e^{(q)} : \langle \boldsymbol{P}\rangle(\mathbf{x}) \tag{S37}$$

with an incident strain field (S3). When the effective-medium description is valid, the local homogenized relation (S37) can be obtained from (S21) by using the following mapping

$$\boldsymbol{C}_p \to \boldsymbol{C}_e\left(k_{L_q}\right),\ \mathcal{I}^{(p)}(\mathbf{x}) \to 1,$$

and thus

$$\boldsymbol{L}_e^{(q)}\left(k_{L_q}\right) \equiv \left[\boldsymbol{C}_e\left(k_{L_q}\right) - \boldsymbol{C}_q\right]/\rho_e : \left[\boldsymbol{I} + \boldsymbol{D}^{(q)} : \left(\boldsymbol{C}_e\left(k_{L_q}\right) - \boldsymbol{C}_q\right)/\rho_e\right]^{-1}. \tag{S38}$$

For this purpose, we first find explicit expressions for $\langle \boldsymbol{P}\rangle(\mathbf{x})$ and $\langle \boldsymbol{f}\rangle(\mathbf{x})$ in terms of the applied field $\boldsymbol{\epsilon}_0$ from the integral equation (S19). We then find an explicit expression for the effective constant tensor $\boldsymbol{L}_e^{(q)}$ by eliminating $\boldsymbol{\epsilon}_0$ between these two expressions. Keeping in mind that the tensors $\boldsymbol{L}^{(q)}$, $\boldsymbol{L}_e^{(q)}$, and $\boldsymbol{H}^{(q)}$ are associated with the reference phase $q$, we shall temporarily drop the superscript $q$ when referring these tensors in the ensuing derivation.

We rewrite (S19) in a compact linear operator form:

$$\boldsymbol{f} = \boldsymbol{\epsilon_0} + \boldsymbol{H}\,\boldsymbol{P}\,. \tag{S39}$$

Combination of this equation with (S21) yields

$$\boldsymbol{P} = \boldsymbol{\mathcal{L}}\,\boldsymbol{\epsilon_0} + \boldsymbol{\mathcal{L}}\,\boldsymbol{H}\,\boldsymbol{P}\,. \tag{S40}$$

The desired relation between $\boldsymbol{P}$ and $\boldsymbol{\epsilon}_0$ can be obtained by iteratively substituting (S40)

$$\boldsymbol{P} = \left(\boldsymbol{I} + \boldsymbol{\mathcal{L}}\,\boldsymbol{H} + \boldsymbol{\mathcal{L}}\,\boldsymbol{H}\,\boldsymbol{\mathcal{L}}\,\boldsymbol{H} + \cdots\right)\boldsymbol{\mathcal{L}}\,\boldsymbol{\epsilon_0} = \left[\boldsymbol{I} - \boldsymbol{\mathcal{L}}\,\boldsymbol{H}\right]^{-1}\boldsymbol{\mathcal{L}}\,\boldsymbol{\epsilon_0} = \boldsymbol{T}\,\boldsymbol{\epsilon_0}\,, \tag{S41}$$

which writes out more explicitly as

$$\begin{aligned}\boldsymbol{P}(\mathbf{1}) =& \boldsymbol{\mathcal{L}}(\mathbf{1}) : \boldsymbol{\epsilon_0}(\mathbf{1}) + \int_\epsilon \mathrm{d}\mathbf{1}'\,\boldsymbol{\mathcal{L}}(\mathbf{1}) : \boldsymbol{H}(\mathbf{1},\mathbf{1}') : \boldsymbol{\mathcal{L}}(\mathbf{1}') : \boldsymbol{\epsilon_0}(\mathbf{1}') \\ &+ \int_\epsilon \mathrm{d}\mathbf{2}\,\mathrm{d}\mathbf{1}'\,\boldsymbol{\mathcal{L}}(\mathbf{1}) : \boldsymbol{H}(\mathbf{1},\mathbf{2}) : \boldsymbol{\mathcal{L}}(\mathbf{2}) : \boldsymbol{H}(\mathbf{2},\mathbf{1}') : \boldsymbol{\mathcal{L}}(\mathbf{1}') : \boldsymbol{\epsilon_0}(\mathbf{1}') + \cdots \\ =& \int_\epsilon \mathrm{d}\mathbf{1}'\,\boldsymbol{T}(\mathbf{1},\mathbf{1}') : \boldsymbol{\epsilon_0}(\mathbf{1}')\,,\end{aligned} \tag{S42}$$

where the boldface numbers $\mathbf{1},\mathbf{2},\cdots$ are short-hand notations for position vectors $\mathbf{r}_1,\mathbf{r}_2,\cdots$. For a statistically homogeneous medium, an ensemble average of the two-point operator $\boldsymbol{T}(\mathbf{1},\mathbf{1}')$ becomes dependent on relative positions, i.e., $\langle \boldsymbol{T}\rangle(\mathbf{1},\mathbf{1}') = \langle \boldsymbol{T}\rangle(\mathbf{1}-\mathbf{1}')$, and an ensemble average of Eq. (S42) can be written as a convolution:

$$\langle \boldsymbol{P}\rangle(\mathbf{1}) = \int_\epsilon \mathrm{d}\mathbf{1}'\,\langle \boldsymbol{T}\rangle(\mathbf{1}-\mathbf{1}') : \boldsymbol{\epsilon_0}(\mathbf{1}')\,. \tag{S43}$$

The two-point operator $\langle \boldsymbol{T}\rangle(\mathbf{1}-\mathbf{1}')$ is explicitly written as

$$\begin{aligned}\langle \boldsymbol{T}\rangle(\mathbf{1}-\mathbf{1}') =& \Big[\boldsymbol{I}\left\langle \mathcal{I}^{(p)}(\mathbf{1})\right\rangle + \boldsymbol{L} : \boldsymbol{H}(\mathbf{1}-\mathbf{1}')\left\langle \mathcal{I}^{(p)}(\mathbf{1})\,\mathcal{I}^{(p)}(\mathbf{1}')\right\rangle \\ &+ \int_\epsilon \mathrm{d}\mathbf{2}\,\boldsymbol{L} : \boldsymbol{H}(\mathbf{1}-\mathbf{2}) : \boldsymbol{L} : \boldsymbol{H}(\mathbf{2}-\mathbf{1}')\left\langle \mathcal{I}^{(p)}(\mathbf{1})\,\mathcal{I}^{(p)}(\mathbf{2})\,\mathcal{I}^{(p)}(\mathbf{1}')\right\rangle + \cdots\Big] : \boldsymbol{L} \\ =& \Big[\boldsymbol{I}\,S_1^{(p)}(\mathbf{1}) + \boldsymbol{U}(\mathbf{1}-\mathbf{1}')\,S_2^{(p)}(\mathbf{1},\mathbf{1}') + \int_\epsilon \mathrm{d}\mathbf{2}\,\boldsymbol{U}(\mathbf{1}-\mathbf{2}) : \boldsymbol{U}(\mathbf{2}-\mathbf{1}')\,S_3^{(p)}(\mathbf{1},\mathbf{2},\mathbf{1}') \\ &+ \cdots\Big] : \boldsymbol{L}\,,\end{aligned} \tag{S44}$$

where $\boldsymbol{U}(\mathbf{r}) \equiv \boldsymbol{L} : \boldsymbol{H}(\mathbf{r})$, and $S_n^{(p)}(\mathbf{1},\cdots,\mathbf{1}')$ is the $n$-point correlation function of phase $p$ ($\neq q$) (see Sec. II in the main text). Importantly, the relation (S43) is *nonlocal in space* [i.e., $\langle \boldsymbol{P}\rangle(\mathbf{x})$ at $\mathbf{x}$ depends on $\boldsymbol{\epsilon_0}(\mathbf{x}')$ at different positions around $\mathbf{x}$] in general. In the quasistatic regime, however, the applied strain tensor will barely change over the correlation length scales over which $\langle \boldsymbol{T}\rangle(\mathbf{1}-\mathbf{1}')$ vanishes, allowing us to approximate (S43) as follows:

$$\langle \boldsymbol{P}\rangle(\mathbf{1}) \approx \left[\int_\epsilon \mathrm{d}\mathbf{1}' \,\langle \boldsymbol{T}\rangle(\mathbf{1}-\mathbf{1}')\right] : \boldsymbol{\epsilon_0}(\mathbf{1})\,. \tag{S45}$$

We obtain a local homogenized constitutive relation between $\langle \boldsymbol{f}\rangle(\mathbf{x})$ and $\langle \boldsymbol{P}\rangle(\mathbf{x})$ by eliminating the term $\boldsymbol{\epsilon}_0(\mathbf{x})$ in (S39) by substituting (S45):

$$\langle \boldsymbol{f}\rangle = \boldsymbol{\epsilon_0} + \boldsymbol{H}\langle \boldsymbol{P}\rangle = \left(\langle \boldsymbol{T}\rangle^{-1} + \boldsymbol{H}\right)\langle \boldsymbol{P}\rangle\,. \tag{S46}$$

Comparing (S46) with (S37) gives

$$\left[\boldsymbol{L}_e^{(q)}\left(k_{L_q}\right)\right]^{-1} = \langle \boldsymbol{T}\rangle^{-1} + \boldsymbol{H}\,, \tag{S47}$$

which can be written explicitly as

$$\begin{aligned}
\boldsymbol{L} : \left[\boldsymbol{L}_e^{(q)}\left(k_{L_q}\right)\right]^{-1} &= \boldsymbol{L} : \left\{\left[\int_\epsilon \mathrm{d}\mathbf{1}'\,\langle \boldsymbol{T}\rangle(\mathbf{1}-\mathbf{1}')\right]^{-1} + \int_\epsilon \mathrm{d}\mathbf{1}'\,\boldsymbol{H}(\mathbf{1}-\mathbf{1}')\right\}\\
=&\frac{\boldsymbol{I}}{S_1^{(p)}(\mathbf{1})} - \int_\epsilon \mathrm{d}\mathbf{1}'\,\boldsymbol{U}(\mathbf{1},\mathbf{1}')\left[\frac{S_2^{(p)}(\mathbf{1},\mathbf{1}') - S_1^{(p)}(\mathbf{1})\,S_1^{(p)}(\mathbf{1}')}{S_1^{(p)}(\mathbf{1})\,S_1^{(p)}(\mathbf{1}')}\right]\\
&- \int_\epsilon \mathrm{d}\mathbf{2}\,\mathrm{d}\mathbf{1}'\,\boldsymbol{U}(\mathbf{1},\mathbf{2}) : \boldsymbol{U}(\mathbf{2},\mathbf{1}')\left[\frac{S_3^{(p)}(\mathbf{1},\mathbf{2},\mathbf{1}') - S_2^{(p)}(\mathbf{1},\mathbf{2})\,S_2^{(p)}(\mathbf{2},\mathbf{1}')\,/\,S_1^{(p)}(\mathbf{2})}{S_1^{(p)}(\mathbf{1})\,S_1^{(p)}(\mathbf{1}')}\right]\\
&- \int_\epsilon \mathrm{d}\mathbf{2}\,\mathrm{d}\mathbf{3}\,\mathrm{d}\mathbf{1}'\,\boldsymbol{U}(\mathbf{1},\mathbf{2}) : \boldsymbol{U}(\mathbf{2},\mathbf{3}) : \boldsymbol{U}(\mathbf{3},\mathbf{1}')\,\frac{1}{S_1^{(p)}(\mathbf{1})\,S_1^{(p)}(\mathbf{2})\,S_1^{(p)}(\mathbf{3})\,S_1^{(p)}(\mathbf{1}')}\\
&\times [S_1^{(p)}(\mathbf{2})\,S_1^{(p)}(\mathbf{3})\,S_4^{(p)}(\mathbf{1},\mathbf{2},\mathbf{3},\mathbf{1}') - S_1^{(p)}(\mathbf{2})\,S_2^{(p)}(\mathbf{1},\mathbf{2})\,S_3^{(p)}(\mathbf{2},\mathbf{3},\mathbf{1}') - S_1^{(p)}(\mathbf{3})\,S_3^{(p)}(\mathbf{1},\mathbf{2},\mathbf{3})\,S_2^{(p)}(\mathbf{3},\mathbf{1}')\\
&+ S_2^{(p)}(\mathbf{1},\mathbf{2})\,S_2^{(p)}(\mathbf{2},\mathbf{3})\,S_2^{(p)}(\mathbf{3},\mathbf{1}')] + \cdots\,.
\end{aligned} \tag{S48}$$

This series expansion can be rewritten as

$${\phi_p}^2\,\boldsymbol{L}^{(q)} : \left[\boldsymbol{L}_e^{(q)}\left(k_{L_q}\right)\right]^{-1} = \phi_p\,\boldsymbol{I} - \sum_{n=2}^{\infty}\boldsymbol{B}_n^{(p)}\left(k_{L_q}\right), \tag{S49}$$

where

$$\boldsymbol{B}_2^{(p)}\left(k_{L_q}\right) = \int_\epsilon d\mathbf{r}\,\boldsymbol{U}^{(q)}(\mathbf{r})\,\chi_V(\mathbf{r})\,, \tag{S50}$$

$$\begin{aligned}
\boldsymbol{B}_n^{(p)}\left(k_{L_q}\right) =&(-1)^n(\phi_p)^{-(n-2)}\int d\mathbf{x}_2\cdots d\mathbf{x}_n\,\boldsymbol{U}^{(q)}(\mathbf{x}_1-\mathbf{x}_2) : \boldsymbol{U}^{(q)}(\mathbf{x}_{n-1}-\mathbf{x}_n) : \cdots : \boldsymbol{U}^{(q)}(\mathbf{x}_{n-1}-\mathbf{x}_n)\\
&\times \Delta_n^{(p)}(\mathbf{x}_1,\cdots,\mathbf{x}_n)\,,\quad n\geq 3,
\end{aligned} \tag{S51}$$

and $\Delta_n^{(p)}(\mathbf{x}_1,\cdots,\mathbf{x}_n)$ is defined in Sec. II in the main text.

### C. Local Strong-Contrast Expansions for Macroscopically Isotropic Media

Here we assume that the composite is macroscopically isotropic, i.e.,

$$\boldsymbol{C}_e\left(k_{L_q}\right) \equiv d\,K_e\!\left(k_{L_q}\right)\boldsymbol{\Lambda}_h + 2\,G_e\!\left(k_{L_q}\right)\boldsymbol{\Lambda}_s\,,$$

and thus the series expansion (S49) can be rewritten as

$${\phi_p}^2\left[\frac{\kappa_{pq}}{\kappa_{eq}\left(k_{L_q}\right)}\boldsymbol{\Lambda}_h + \frac{\mu_{pq}}{\mu_{eq}\left(k_{L_q}\right)}\boldsymbol{\Lambda}_s\right] = \phi_p\,\boldsymbol{I} - \sum_{n=2}^{\infty}\boldsymbol{B}_n^{(p)}\left(k_{L_q}\right). \tag{S52}$$

Using properties of the projection tensors $\mathbf{\Lambda}_h$ and $\mathbf{\Lambda}_s$ (Sec. III B) yields the strong-contrast expansions for the effective bulk and shear moduli given respectively as

$$\kappa_{eq}\left(k_{L_q}\right) = \frac{K_e\left(k_{L_q}\right) - K_q}{K_e\left(k_{L_q}\right) + 2(d-1)G_q/d} = \frac{{\phi_p}^2 \kappa_{pq}}{\phi - \sum_{n=2}^{\infty} C_n^{(p)}\left(k_{L_q}\right)}, \tag{S53}$$

$$\mu_{eq}\left(k_{L_q}\right) = \frac{G_e\left(k_{L_q}\right) - G_q}{G_e\left(k_{L_q}\right) + [dK_q/2 + (d+1)(d-2)G_q/d]G_q/(K_q + 2G_q)} = \frac{{\phi_p}^2 \mu_{pq}}{\phi_p - \sum_{n=2}^{\infty} D_n^{(p)}\left(k_{L_q}\right)}, \tag{S54}$$

where $C_n^{(p)}\left(k_{L_q}\right) \equiv \boldsymbol{B}_n^{(p)}\left(k_{L_q}\right) \vdots \mathbf{\Lambda}_h$ and $D_n^{(p)}\left(k_{L_q}\right) \equiv 2[(d+2)(d-1)]^{-1}\, \boldsymbol{B}_n^{(p)}\left(k_{L_q}\right) \vdots \mathbf{\Lambda}_s$. In what follows, we derive explicit formulas of $C_n^{(p)}\left(k_{L_q}\right)$ and $D_n^{(p)}\left(k_{L_q}\right)$ for $n = 2, 3$.

### *1. Approximation at the two-point level*

Here we derive the explicit formulas for $C_2^{(p)}\left(k_{L_q}\right)$ and $D_2^{(p)}\left(k_{L_q}\right)$ that are important for the local strong-contrast approximation at the two-point level. To do so, we remind the formulas for $C_2^{(p)}\left(k_{L_q}\right)$, $D_2^{(p)}\left(k_{L_q}\right)$, and $\boldsymbol{U}^{(q)}(\mathbf{r})$. From (S50), the two-point parameters are written respectively as

$$C_2^{(p)}\left(k_{L_q}\right) \equiv \boldsymbol{B}_{\boldsymbol{2}}^{(\boldsymbol{p})}\left(k_{L_q}\right) \vdots \mathbf{\Lambda}_h = \frac{1}{d}\int \mathrm{d}\mathbf{r}\, U_{iikk}^{(q)}(\mathbf{r})\, \chi_V(\mathbf{r}), \tag{S55}$$

$$D_2^{(p)}\left(k_{L_q}\right) \equiv \frac{2}{(d+2)(d-1)}\, \boldsymbol{B}_{\boldsymbol{2}}^{(\boldsymbol{p})}\left(k_{L_q}\right) \vdots \mathbf{\Lambda}_s = \frac{2}{(d+2)(d-1)} \int \mathrm{d}\mathbf{r} \left[U_{ikik}^{(q)}(\mathbf{r}) - \frac{1}{d} U_{iikk}^{(q)}(\mathbf{r})\right] \chi_V(\mathbf{r}), \tag{S56}$$

where

$$\begin{aligned} U_{ijkl}^{(q)}(\mathbf{r}) \equiv& L_{ijmn}^{(q)} H_{mnkl}^{(q)}(\mathbf{r}) \\ =& d{c_{L_q}}^2 \left[\left(\kappa_{pq} - \frac{(d+2){c_{T_q}}^2}{d{c_{L_q}}^2 + 2{c_{T_q}}^2}\mu_{pq}\right)\frac{1}{d}\,\delta_{ij}\, H_{mmkl}^{(q)}(\mathbf{r}) + \frac{(d+2){c_{T_q}}^2}{d{c_{L_q}}^2 + 2{c_{T_q}}^2}\mu_{pq}\, H_{ijkl}^{(q)}(\mathbf{r})\right], \end{aligned} \tag{S57}$$

and $\boldsymbol{H}^{(q)}(\mathbf{r})$ is given in Eq. (S26).

To compute (S55) and (S56), we first obtain $U_{iikk}^{(q)}(\mathbf{r})$ and $U_{ikik}^{(q)}(\mathbf{r})$ from (S57)

$$\begin{aligned} U_{iikk}^{(q)}(\mathbf{r}) =& d{c_{L_q}}^2 \left[\left(\kappa_{pq} - \frac{(d+2){c_{T_q}}^2}{d{c_{L_q}}^2 + 2{c_{T_q}}^2}\mu_{pq}\right) H_{mmkk}^{(q)}(\mathbf{r}) + \frac{(d+2){c_{T_q}}^2}{d{c_{L_q}}^2 + 2{c_{T_q}}^2}\mu_{pq}\, H_{iikk}^{(q)}(\mathbf{r})\right] \\ =& d{c_{L_q}}^2 \kappa_{pq}\, H_{iikk}^{(q)}(\mathbf{r}) = -\frac{id\pi}{2(2\pi)^{d/2}} \frac{{c_{L_q}}^2}{\omega^2 r^{d+2}} \kappa_{pq} {r_L}^{d/2+3}\, \mathcal{H}_{d/2-1}^{(1)}(r_L), \end{aligned} \tag{S58}$$

$$\begin{aligned} U_{ikik}^{(q)}(\mathbf{r}) =& d{c_{L_q}}^2 \left[\left(\kappa_{pq} - \frac{(d+2){c_{T_q}}^2}{d{c_{L_q}}^2 + 2{c_{T_q}}^2}\mu_{pq}\right)\frac{1}{d} H_{mmkk}^{(q)}(\mathbf{r}) + \frac{(d+2){c_{T_q}}^2}{d{c_{L_q}}^2 + 2{c_{T_q}}^2}\mu_{pq}\, H_{ikik}^{(q)}(\mathbf{r})\right] \\ =& \frac{1}{d} U_{iikk}^{(q)}(\mathbf{r}) + d{c_{L_q}}^2 \frac{(d+2){c_{T_q}}^2}{d{c_{L_q}}^2 + 2{c_{T_q}}^2}\mu_{pq} \left[H_{ikik}^{(q)}(\mathbf{r}) - \frac{1}{d} H_{iikk}^{(q)}(\mathbf{r})\right] \\ =& \frac{1}{d} U_{iikk}^{(q)}(\mathbf{r}) - \frac{id\pi}{2(2\pi)^{d/2}} \frac{(d-1)(d+2)}{d{c_{L_q}}^2 + 2{c_{T_q}}^2} \frac{{c_{L_q}}^2 {c_{T_q}}^2}{\omega^2 r^{d+2}} \mu_{pq} \left[\frac{1}{d}{r_L}^{d/2+3}\, \mathcal{H}_{d/2-1}^{(1)}(r_L) + \frac{1}{2}{r_T}^{d/2+3}\, \mathcal{H}_{d/2-1}^{(1)}(r_T)\right], \end{aligned} \tag{S59}$$

where we have used the properties of $\boldsymbol{H}^{(q)}(\mathbf{r})$ (cf. Sec. III C), $r_L \equiv k_{L_q} r$, and $r_T \equiv k_{T_q} r$. Using (S58) and (S59), we

simplify Eqs. (S55) and (S56) as follow:

$$C_2^{(p)}(k_{L_q}) = \frac{\pi}{2^{d/2}\,\Gamma(d/2)}\kappa_{pq}\left[-i\int_0^\infty \mathrm{d}r\,(k_{L_q} r)^{d/2}\,k_{L_q}\,\mathcal{H}^{(1)}_{d/2-1}(k_{L_q} r)\,\chi_V(r)\right] = \frac{\pi}{2^{d/2}\,\Gamma(d/2)}\kappa_{pq}\,\mathcal{F}(k_{L_q}) \tag{S60}$$

$$\begin{aligned} D_2^{(p)}(k_{L_q}) =& \frac{\pi}{2^{d/2}\,\Gamma(d/2)}\frac{2d}{d{c_{L_q}}^2+2{c_{T_q}}^2}\mu_{pq}\left[-\frac{{c_{T_q}}^2}{d}i\int_0^\infty \mathrm{d}r\,(k_{L_q} r)^{d/2}\,k_{L_q}\,\mathcal{H}^{(1)}_{d/2-1}(k_{L_q} r)\right. \\ &\left. -\frac{{c_{L_q}}^2}{2}i\int_0^\infty \mathrm{d}r\,(k_{T_q} r)^{d/2}\,k_{T_q}\,\mathcal{H}^{(1)}_{d/2-1}(k_{T_q} r)\right] \\ =& \frac{\pi}{2^{d/2}\,\Gamma(d/2)}\left[\frac{2\,{c_{T_q}}^2\,\mathcal{F}(k_{L_q})+d\,{c_{L_q}}^2\,\mathcal{F}(k_{T_q})}{d{c_{L_q}}^2+2{c_{T_q}}^2}\right]\mu_{pq}, \end{aligned} \tag{S61}$$

where $\Gamma(x)$ is the Gamma function, and the *local attenuation function* $\mathcal{F}(Q)$ is defined as

$$\mathcal{F}(Q) \equiv -\frac{2^{d/2}\,\Gamma(d/2)}{\pi}Q^2\int_\epsilon \frac{i}{4}\left(\frac{Q}{2\pi r}\right)^{d/2-1}\mathcal{H}^{(1)}_{d/2-1}(Qr)\,\chi_V(r)\,\mathrm{d}\mathbf{r} \tag{S62}$$

$$= -\frac{\Gamma(d/2)}{2^{d/2}\pi^{d+1}}Q^2\int \frac{\tilde{\chi}_V(\mathbf{q})}{|\mathbf{q}|^2-Q^2}\,\mathrm{d}\mathbf{q}\,, \tag{S63}$$

and Eq. (S63) is obtained by applying the Parseval theorem to Eq. (S62). The real and imaginary parts of $\mathcal{F}(Q)$ are respectively given as

$$\mathrm{Im}[\mathcal{F}(Q)] = -\lim_{\epsilon\to 0^+}\int_\epsilon^\infty \mathrm{d}r\,Q\,\chi_V(r)\,(Qr)^{d/2}\,J_{d/2-1}(Qr) \tag{S64}$$

$$= -\frac{Q^d}{(2\pi)^{d/2}}\,\tilde{\chi}_V(Q)\,, \tag{S65}$$

$$\mathrm{Re}[\mathcal{F}(Q)] = \lim_{\epsilon\to 0^+}\int_\epsilon^\infty \mathrm{d}r\,Q\,\chi_V(r)\,(Qr)^{d/2}\,Y_{d/2-1}(Qr) \tag{S66}$$

$$= -\frac{2Q^2}{\pi}\mathrm{p.v.}\int_0^\infty \mathrm{d}q\,\frac{1}{q(Q^2-q^2)}\,\mathrm{Im}[\mathcal{F}(q)], \tag{S67}$$

where $J_\nu(x)$ [$Y_\nu(x)$] is the Bessel function of the first kind [the second kind] of order $\nu$, and p.v. stands for the Cauchy principal value of an integral.

### 2. *Approximation at the three-point level*

Here we derive the explicit formulas for $C_3^{(p)}(k_{L_q})$ and $D_3^{(p)}(k_{L_q})$ that are important for the local strong-contrast approximation at the three-point level. These three-point parameters are defined respectively as

$$\begin{aligned} C_3^{(p)}(k_{L_q}) \equiv& \boldsymbol{B}_3^{(p)}(k_{L_q}) ⋮ \boldsymbol{\Lambda}_h \\ =& \frac{-1}{\phi_p}\int_\epsilon d\mathbf{2}\,d\mathbf{3}\left[\boldsymbol{U}^{(q)}(\mathbf{1}-\mathbf{2}) : \boldsymbol{U}^{(q)}(\mathbf{2}-\mathbf{3})\right] ⋮ \boldsymbol{\Lambda}_h\,\Delta_3^{(p)}(\mathbf{1},\mathbf{2},\mathbf{3})\,, \end{aligned} \tag{S68}$$

$$\begin{aligned} D_3^{(p)}(k_{L_q}) \equiv& \frac{2}{(d+2)(d-1)}\boldsymbol{B}_3^{(p)}(k_{L_q}) ⋮ \boldsymbol{\Lambda}_s \\ =& \frac{2}{(d+2)(d-1)}\frac{-1}{\phi_p}\int_\epsilon d\mathbf{2}\,d\mathbf{3}\left[\boldsymbol{U}^{(q)}(\mathbf{1}-\mathbf{2}) : \boldsymbol{U}^{(q)}(\mathbf{2}-\mathbf{3})\right] ⋮ \boldsymbol{\Lambda}_s\,\Delta_3^{(p)}(\mathbf{1},\mathbf{2}.\mathbf{3})\,, \end{aligned} \tag{S69}$$

respectively. To do so, we first obtain expressions for $\boldsymbol{U}^{(q)}(\mathbf{r}):\boldsymbol{U}^{(q)}(\mathbf{s})$ from (S57):

$$U^{(q)}_{ijmn}(\mathbf{r})\,U^{(q)}_{mnkl}(\mathbf{s})=\left(d{c_{L_q}}^2\right)^2\Bigg\{\left(\kappa_{pq}-\frac{(d+2){c_{T_q}}^2}{d{c_{L_q}}^2+2{c_{T_q}}^2}\mu_{pq}\right)^2\frac{1}{d^2}\,\delta_{ij}\,H^{(q)}_{mmnn}(\mathbf{r})\,H^{(q)}_{m'm'kl}(\mathbf{s})$$
$$+\frac{(d+2){c_{T_q}}^2}{d{c_{L_q}}^2+2{c_{T_q}}^2}\mu_{pq}\left(\kappa_{pq}-\frac{(d+2){c_{T_q}}^2}{d{c_{L_q}}^2+2{c_{T_q}}^2}\mu_{pq}\right)\frac{1}{d}\left[\delta_{ij}\,H^{(q)}_{m'm'mn}(\mathbf{r})\,H^{(q)}_{mnkl}(\mathbf{s})+H^{(q)}_{ijmm}(\mathbf{r})\,H^{(q)}_{nnkl}(\mathbf{s})\right]$$
$$+\left(\frac{(d+2){c_{T_q}}^2}{d{c_{L_q}}^2+2{c_{T_q}}^2}\mu_{pq}\right)^2H^{(q)}_{ijmn}(\mathbf{r})\,H^{(q)}_{mnkl}(\mathbf{s})\Bigg\}.\tag{S70}$$

Using (S70), we obtain

$$\left[\boldsymbol{U}^{(q)}(\mathbf{r}):\boldsymbol{U}^{(q)}(\mathbf{s})\right]\vdots\,\boldsymbol{\Lambda_h}=(\Lambda_h)_{ijkl}\,U^{(q)}_{ijmn}(\mathbf{r})\,U^{(q)}_{mnkl}(\mathbf{s})$$
$$=\frac{\left(d{c_{L_q}}^2\right)^2}{d}\Bigg\{\left[\kappa_{pq}-\frac{(d+2){c_{T_q}}^2}{d{c_{L_q}}^2+2{c_{T_q}}^2}\mu_{pq}\right]^2\frac{1}{d}\,H^{(q)}_{mmnn}(\mathbf{r})\,H^{(q)}_{m'm'n'n'}(\mathbf{s})$$
$$+\frac{(d+2){c_{T_q}}^2}{d{c_{L_q}}^2+2{c_{T_q}}^2}\mu_{pq}\left[\kappa_{pq}-\frac{(d+2){c_{T_q}}^2}{d{c_{L_q}}^2+2{c_{T_q}}^2}\mu_{pq}\right]\frac{1}{d}\left[d\,H^{(q)}_{m'm'mn}(\mathbf{r})\,H^{(q)}_{mnkk}(\mathbf{s})+H^{(q)}_{n'n'mm}(\mathbf{r})\,H^{(q)}_{nnm'm'}(\mathbf{s})\right]$$
$$+\left(\frac{(d+2){c_{T_q}}^2}{d{c_{L_q}}^2+2{c_{T_q}}^2}\mu_{pq}\right)^2H^{(q)}_{llmn}(\mathbf{r})\,H^{(q)}_{mnkk}(\mathbf{s})\Bigg\}$$
$$=\frac{\left(d{c_{L_q}}^2\right)^2}{d}\Bigg\{\left(\kappa_{pq}-\frac{(d+2){c_{T_q}}^2}{d{c_{L_q}}^2+2{c_{T_q}}^2}\mu_{pq}\right)\kappa_{pq}\frac{1}{d}\,H^{(q)}_{iijj}(\mathbf{r})\,H^{(q)}_{i'i'j'j'}(\mathbf{s})$$
$$+\frac{(d+2){c_{T_q}}^2}{d{c_{L_q}}^2+2{c_{T_q}}^2}\mu_{pq}\kappa_{pq}\,H^{(q)}_{iikl}(\mathbf{r})\,H^{(q)}_{kli'i'}(\mathbf{s})\Bigg\}.\tag{S71}$$

Substituting the expressions for $\boldsymbol{H}^{(q)}(\mathbf{r})$ in Sec. III C into (S71) gives

$$\left[\boldsymbol{U}^{(q)}(\mathbf{r}):\boldsymbol{U}^{(q)}(\mathbf{s})\right]\vdots\,\boldsymbol{\Lambda_h}$$
$$=-\frac{d\pi^2}{4(2\pi)^d}\frac{{k_{L_q}}^d}{\sqrt{rs}^d}\Bigg\{\left[\kappa_{pq}-\frac{(d+2){c_{T_q}}^2}{d{c_{L_q}}^2+2{c_{T_q}}^2}\mu_{pq}\right]\kappa_{pq}\frac{1}{d}(k_{L_q}r)\,\mathcal{H}^{(1)}_{d/2-1}(k_{L_q}r)\,(k_{L_q}s)\,\mathcal{H}^{(1)}_{d/2-1}(k_{L_q}s)$$
$$+\frac{(d+2){c_{T_q}}^2}{d{c_{L_q}}^2+2{c_{T_q}}^2}\mu_{pq}\kappa_{pq}\Big[d\,\mathcal{H}^{(1)}_{d/2}(k_{L_q}r)\,\mathcal{H}^{(1)}_{d/2}(k_{L_q}s)-\mathcal{H}^{(1)}_{d/2}(k_{L_q}r)\,(k_{L_q}s)\,\mathcal{H}^{(1)}_{d/2+1}(k_{L_q}s)$$
$$-(k_{L_q}r)\,\mathcal{H}^{(1)}_{d/2+1}(k_{L_q}r)\,\mathcal{H}^{(1)}_{d/2}(k_{L_q}s)+(\hat{\mathbf{r}}\cdot\hat{\mathbf{s}})^2(k_{L_q}r)\,\mathcal{H}^{(1)}_{d/2+1}(k_{L_q}r)\,(k_{L_q}s)\,\mathcal{H}^{(1)}_{d/2+1}(k_{L_q}s)\Big]\Bigg\}\tag{S72}$$
$$=-\frac{d\pi^2}{4(2\pi)^d}\frac{{k_{L_q}}^d}{\sqrt{rs}^d}\Bigg(\left[\kappa_{pq}-\frac{(d+2){c_{T_q}}^2}{d{c_{L_q}}^2+2{c_{T_q}}^2}\mu_{pq}\right]\kappa_{pq}\frac{1}{d}(k_{L_q}r)\,\mathcal{H}^{(1)}_{d/2-1}(k_{L_q}r)\,(k_{L_q}s)\,\mathcal{H}^{(1)}_{d/2-1}(k_{L_q}s)$$
$$+\frac{(d+2){c_{T_q}}^2}{d{c_{L_q}}^2+2{c_{T_q}}^2}\mu_{pq}\kappa_{pq}\Big\{\frac{1}{d}(k_{L_q}r)\,\mathcal{H}^{(1)}_{d/2-1}(k_{L_q}r)\,(k_{L_q}s)\,\mathcal{H}^{(1)}_{d/2-1}(k_{L_q}s)$$
$$+\frac{1}{d}\left[d(\hat{\mathbf{r}}\cdot\hat{\mathbf{s}})^2-1\right](k_{L_q}r)\,\mathcal{H}^{(1)}_{d/2+1}(k_{L_q}r)\,(k_{L_q}s)\,\mathcal{H}^{(1)}_{d/2+1}(k_{L_q}s)\Big\}\Bigg)$$
$$=-\frac{\pi^2}{4(2\pi)^d}\frac{{k_{L_q}}^{d+2}}{\sqrt{rs}^{d-2}}\kappa_{pq}\Bigg\{\kappa_{pq}\,\mathcal{H}^{(1)}_{d/2-1}(k_{L_q}r)\,\mathcal{H}^{(1)}_{d/2-1}(k_{L_q}s)$$
$$+\frac{(d+2){c_{T_q}}^2}{d{c_{L_q}}^2+2{c_{T_q}}^2}\mu_{pq}\left[d(\hat{\mathbf{r}}\cdot\hat{\mathbf{s}})^2-1\right]\mathcal{H}^{(1)}_{d/2+1}(k_{L_q}r)\,\mathcal{H}^{(1)}_{d/2+1}(k_{L_q}s)\Bigg\},\tag{S73}$$

where we have used the recurrence relation of $\mathcal{H}_\nu^{(1)}(x)$; see (S104). Use of (S68) and (S73) yields

$$C_3^{(p)}(k_{L_q}) = -\frac{\pi^2 {k_{L_q}}^{d+2}}{4(2\pi)^d}\kappa_{pq}\int_\epsilon \frac{\mathrm{d}\mathbf{r}}{r^{d/2-1}}\int_\epsilon \frac{\mathrm{d}\mathbf{s}}{s^{d/2-1}}\Bigg\{\kappa_{pq}\,\mathcal{H}_{d/2-1}^{(1)}(k_{L_q} r)\,\mathcal{H}_{d/2-1}^{(1)}(k_{L_q} s) + \frac{(d+2){c_{T_q}}^2}{d{c_{L_q}}^2+2{c_{T_q}}^2}\mu_{pq}\big[d(\hat{\mathbf{r}}\cdot\hat{\mathbf{s}})^2-1\big]\,\mathcal{H}_{d/2+1}^{(1)}(k_{L_q} r)\,\mathcal{H}_{d/2+1}^{(1)}(k_{L_q} s)\Bigg\} \times\left[S_3^{(p)}(\mathbf{r},\mathbf{s},\mathbf{t}) - \frac{S_2^{(p)}(\mathbf{r})\,S_2^{(p)}(\mathbf{s})}{\phi_p}\right], \tag{S74}$$

where $\mathbf{t}\equiv\mathbf{r}-\mathbf{s}$.

Using (S70), we now compute

$$\begin{aligned}\big[\boldsymbol{U}^{(q)}(\mathbf{r}):\boldsymbol{U}^{(q)}(\mathbf{s})\big]\,\vdots\,\boldsymbol{\Lambda}_s &= U_{ikmn}^{(q)}(\mathbf{r})\,U_{mnik}^{(q)}(\mathbf{s}) - \frac{1}{d}\,U_{iimn}^{(q)}(\mathbf{r})\,U_{mnkk}^{(q)}(\mathbf{s})\\ =&\big(d{c_{L_q}}^2\big)^2\Bigg\{\left[\frac{(d+2){c_{T_q}}^2}{d{c_{L_q}}^2+2{c_{T_q}}^2}\mu_{pq}\right]^2\frac{1}{d^2}\,H_{mmnn}^{(q)}(\mathbf{r})\,H_{m'm'n'n'}^{(q)}(\mathbf{s})\\ &+\frac{(d+2){c_{T_q}}^2}{d{c_{L_q}}^2+2{c_{T_q}}^2}\mu_{pq}\left(\kappa_{pq}-\frac{2(d+2){c_{T_q}}^2}{d{c_{L_q}}^2+2{c_{T_q}}^2}\mu_{pq}\right)\frac{1}{d}\,H_{m'm'mn}^{(q)}(\mathbf{r})\,H_{mnii}^{(q)}(\mathbf{s})\\ &+\left(\frac{(d+2){c_{T_q}}^2}{d{c_{L_q}}^2+2{c_{T_q}}^2}\mu_{pq}\right)^2 H_{ikmn}^{(q)}(\mathbf{r})\,H_{mnik}^{(q)}(\mathbf{s})\Bigg\}.\end{aligned} \tag{S75}$$

Here, the two terms $H_{mmnn}^{(q)}(\mathbf{r})\,H_{m'm'n'n'}^{(q)}(\mathbf{s})$ and $H_{m'm'mn}^{(q)}(\mathbf{r})\,H_{mnii}^{(q)}(\mathbf{s})$ are easy to compute by using formulas in Sec. III C. After some tedious calculations, the last term $H_{ikmn}^{(q)}(\mathbf{r})\,H_{mnik}^{(q)}(\mathbf{s})$ can be rewritten by use of the formulas in Table S2 as follows:

$$H_{ikmn}^{(q)}(\mathbf{r})\,H_{mnik}^{(q)}(\mathbf{s}) = \frac{-\pi^2}{4(2\pi)^d}\frac{1}{r^{d+2}s^{d+2}\omega^4}\big[M_0(r,s)+(\hat{\mathbf{r}}\cdot\hat{\mathbf{s}})^2\,M_2(r,s)+(\hat{\mathbf{r}}\cdot\hat{\mathbf{s}})^4\,M_4(r,s)\big], \tag{S76}$$

where

$$\begin{aligned}M_0(r,s)\equiv&\Big[{r_L}^{d/2+3}\,\mathcal{H}_{d/2+3}^{(1)}(r_L)-{r_T}^{d/2+3}\,\mathcal{H}_{d/2+3}^{(1)}(r_T)\Big]\\ &\times\Big[3{s_L}^{d/2+1}\,\mathcal{H}_{d/2+1}^{(1)}(s_L)-3{s_T}^{d/2+1}\,\mathcal{H}_{d/2+1}^{(1)}(s_T)+{s_T}^{d/2+2}\,\mathcal{H}_{d/2}^{(1)}(s_T)\Big]\\ &+\Big[{r_L}^{d/2+2}\,\mathcal{H}_{d/2+2}^{(1)}(r_L)-{r_T}^{d/2+2}\,\mathcal{H}_{d/2+2}^{(1)}(r_T)\Big]\\ &\times\Big[-6{s_L}^{d/2+2}\,\mathcal{H}_{d/2}^{(1)}(s_L)-2(d-1){s_T}^{d/2+2}\,\mathcal{H}_{d/2}^{(1)}(s_T)+{s_T}^{d/2+3}\,\mathcal{H}_{d/2+1}^{(1)}(s_T)\Big]\\ &+{r_T}^{d/2+3}\,\mathcal{H}_{d/2+1}^{(1)}(r_T)\left[-{s_L}^{d/2+2}\,\mathcal{H}_{d/2}^{(1)}(s_L)-\frac{d-1}{2}{s_T}^{d/2+2}\,\mathcal{H}_{d/2}^{(1)}(s_T)+\frac{1}{4}{s_T}^{d/2+3}\,\mathcal{H}_{d/2+1}^{(1)}(s_T)\right]\\ &+\Big[{r_L}^{d/2+1}\,\mathcal{H}_{d/2+1}^{(1)}(r_L)-{r_T}^{d/2+1}\,\mathcal{H}_{d/2+1}^{(1)}(r_T)\Big]{s_L}^{d/2+3}\,\mathcal{H}_{d/2-1}^{(1)}(s_L)\\ &+\Big[2{r_L}^{d/2+1}\,\mathcal{H}_{d/2+1}^{(1)}(r_L)-2{r_T}^{d/2+1}\,\mathcal{H}_{d/2+1}^{(1)}(r_T)+{r_T}^{d/2+2}\,\mathcal{H}_{d/2}^{(1)}(r_T)\Big]\\ &\times\left[{s_L}^{d/2+3}\,\mathcal{H}_{d/2-1}^{(1)}(s_L)+\frac{d-1}{2}{s_T}^{d/2+3}\,\mathcal{H}_{d/2-1}^{(1)}(s_T)\right],\end{aligned} \tag{S77}$$

$$\begin{aligned}M_2(r,s)\equiv&-\Big[{r_L}^{d/2+3}\,\mathcal{H}_{d/2+3}^{(1)}(r_L)-{r_T}^{d/2+3}\,\mathcal{H}_{d/2+3}^{(1)}(r_T)\Big]\Big[{s_L}^{d/2+2}\,\mathcal{H}_{d/2+2}^{(1)}(s_L)-{s_T}^{d/2+2}\,\mathcal{H}_{d/2+2}^{(1)}(s_T)\Big]\\ &+6\Big[{r_L}^{d/2+2}\,\mathcal{H}_{d/2+2}^{(1)}(r_L)-{r_T}^{d/2+2}\,\mathcal{H}_{d/2+2}^{(1)}(r_T)\Big]\Big[{s_L}^{d/2+3}\,\mathcal{H}_{d/2+1}^{(1)}(s_L)-{s_T}^{d/2+3}\,\mathcal{H}_{d/2+1}^{(1)}(s_T)\Big]\\ &+{r_T}^{d/2+3}\,\mathcal{H}_{d/2+1}^{(1)}(r_T)\,{s_L}^{d/2+3}\,\mathcal{H}_{d/2+1}^{(1)}(s_L)\\ &+\left[{r_L}^{d/2+3}\,\mathcal{H}_{d/2+1}^{(1)}(r_L)-\frac{d-6}{4}{r_T}^{d/2+3}\,\mathcal{H}_{d/2+1}^{(1)}(r_T)\right]{s_T}^{d/2+3}\,\mathcal{H}_{d/2+1}^{(1)}(s_T),\end{aligned} \tag{S78}$$

$$M_4(r,s)\equiv\Big[{r_L}^{d/2+3}\,\mathcal{H}_{d/2+3}^{(1)}(r_L)-{r_T}^{d/2+3}\,\mathcal{H}_{d/2+3}^{(1)}(r_T)\Big]\Big[{s_L}^{d/2+3}\,\mathcal{H}_{d/2+3}^{(1)}(s_L)-{s_T}^{d/2+3}\,\mathcal{H}_{d/2+3}^{(1)}(s_T)\Big], \tag{S79}$$

where $r_L \equiv k_{L_q} r$, $r_T \equiv k_{T_q} r$, $s_T \equiv k_{L_q} s$, and $s_T \equiv k_{T_q} s$. We substitute the newly obtained expression for Eq. (S75) into (S69) and then rearrange it in terms of $\hat{P}_4(\hat{\mathbf{r}}\cdot\hat{\mathbf{s}})$ and $\hat{P}_2(\hat{\mathbf{r}}\cdot\hat{\mathbf{s}})$, where

$$\hat{P}_4(t) \equiv t^4 - \frac{6}{d+4}t^2 + \frac{3}{(d+2)(d+4)}, \tag{S80}$$

$$\hat{P}_2(t) \equiv dt^2 - 1, \tag{S81}$$

which correspond to $d$-dimensional Legendre polynomials of order 4 and 2, respectively, up to the normalization constants. After painstaking algebraic calculations, we derive

$$\begin{aligned} D_3^{(p)}(k_{L_q}) = \frac{2}{d-1}\frac{{k_{L_q}}^{d+2}}{2^{2+d}\pi^{d-2}}\frac{{c_{T_q}}^2\,\mu_{pq}}{d\,{c_{L_q}}^2+2\,{c_{T_q}}^2}\iint\frac{\mathrm{d}\mathbf{r}}{r^{d/2-1}}\frac{\mathrm{d}\mathbf{s}}{s^{d/2-1}}\Bigg(-\kappa_{pq}\,\hat{P}_2(\hat{\mathbf{r}}\cdot\mathbf{s})\,\mathcal{H}^{(1)}_{d/2+1}(k_{L_q}r)\,\mathcal{H}^{(1)}_{d/2+1}(k_{L_q}s) \\ -\frac{(d+2)\,{c_{T_q}}^2\,\mu_{pq}}{d\,{c_{L_q}}^2+2\,{c_{T_q}}^2}\Bigg\{d^2\,\hat{P}_4(\hat{\mathbf{r}}\cdot\mathbf{s})\left[\mathcal{H}^{(1)}_{d/2+3}(k_{L_q}r)-\frac{\mathcal{H}^{(1)}_{d/2+3}(k_{T_q}r)}{(c_{T_q}/c_{L_q})^{d/2+3}}\right]\left[\mathcal{H}^{(1)}_{d/2+3}(k_{L_q}s)-\frac{\mathcal{H}^{(1)}_{d/2+3}(k_{T_q}s)}{(c_{T_q}/c_{L_q})^{d/2+3}}\right] \\ +\frac{d-2}{4(d+4)}\,\hat{P}_2(\hat{\mathbf{r}}\cdot\mathbf{s})\left[4\,\mathcal{H}^{(1)}_{d/2+1}(k_{L_q}r)+d\frac{\mathcal{H}^{(1)}_{d/2+1}(k_{T_q}r)}{(c_{T_q}/c_{L_q})^{d/2+3}}\right]\left[4\,\mathcal{H}^{(1)}_{d/2+1}(k_{L_q}s)+d\frac{\mathcal{H}^{(1)}_{d/2+1}(k_{T_q}s)}{(c_{T_q}/c_{L_q})^{d/2+3}}\right] \\ +\frac{d-1}{2(d+2)}\left[2\,\mathcal{H}^{(1)}_{d/2-1}(k_{L_q}r)+d\frac{\mathcal{H}^{(1)}_{d/2-1}(k_{T_q}r)}{(c_{T_q}/c_{L_q})^{d/2+3}}\right]\left[2\,\mathcal{H}^{(1)}_{d/2-1}(k_{L_q}s)+d\frac{\mathcal{H}^{(1)}_{d/2-1}(k_{T_q}s)}{(c_{T_q}/c_{L_q})^{d/2+3}}\right]\Bigg\}\Bigg) \\ \times\left[S_3^{(p)}(\mathbf{r},\mathbf{s},\mathbf{t})-\frac{S_2^{(p)}(\mathbf{r})\,S_2^{(p)}(\mathbf{s})}{\phi_p}\right]. \end{aligned} \tag{S82}$$

## II. DERIVATION OF GREEN FUNCTIONS FOR AN ISOTROPIC MEDIUM

In this section, we derive the explicit formulas for the Green functions employed in this work.

### A. Dyadic Green Function $\boldsymbol{g}^{(q)}(\mathbf{r})$

Here we derive the explicit expression for the dyadic Green function $g_{ij}^{(q)}(\mathbf{x},\mathbf{x}') = g_{ij}^{(q)}(\mathbf{x}-\mathbf{x}')$ associated with the elastic wave equation considered in Sec. II in the main text. The Green function satisfies the following equation:

$$\omega^2\,g_{ij}^{(q)}(\mathbf{r}) + \left({c_{L_q}}^2-{c_{T_q}}^2\right)\frac{\partial^2\,g_{kj}^{(q)}(\mathbf{r},)}{\partial x_i\partial x_k} + {c_{T_q}}^2\frac{\partial^2\,g_{ij}^{(q)}(\mathbf{r})}{\partial x_l\partial x_l} = -\delta_{ij}\,\delta(\mathbf{r})\,,$$

where $\mathbf{r}\equiv\mathbf{x}-\mathbf{x}'$. We reduce this partial differential equation into a system of linear equations by taking the Fourier transform on the both sides;

$$\begin{aligned} -\delta_{ij} &= \omega^2\,\tilde{g}_{ij}^{(q)}(\mathbf{q}) - \left({c_{L_q}}^2-{c_{T_q}}^2\right)q_iq_k\,\tilde{g}_{kj}^{(q)}(\mathbf{q}) - {c_{T_q}}^2 q_lq_l\,\tilde{g}_{ij}^{(q)}(\mathbf{q}) \\ &= \left[-\left({c_{L_q}}^2-{c_{T_q}}^2\right)q_iq_k + (\omega^2-{c_{T_q}}^2q_lq_l)\delta_{ik}\right]\tilde{g}_{kj}^{(q)}(\mathbf{q}) \\ &= \left[\left(-{c_{L_q}}^2q^2+\omega^2\right)\Pi_{ik} + (\omega^2-{c_{T_q}}^2q^2)\,(\delta_{ik}-\Pi_{ik})\right]\tilde{g}_{kj}^{(q)}(\mathbf{q})\,, \end{aligned} \tag{S83}$$

where $\Pi_{ij}\equiv\hat{\mathbf{q}}_i\hat{\mathbf{q}}_j$ is the projection operator on a given wavevector $\mathbf{q}$. Equation (S83) implies that $\boldsymbol{g}^{(q)}(\mathbf{q})$ is the inverse of $-\left(-{c_{L_q}}^2k^2+\omega^2\right)\boldsymbol{\Pi}-(\omega^2-{c_{T_q}}^2k^2)\,(\boldsymbol{I}-\boldsymbol{\Pi})$, and thus using the following properties of projection operators

$$\boldsymbol{\Pi}\cdot\boldsymbol{\Pi}=\boldsymbol{\Pi}\,,\ \ (\boldsymbol{I}-\boldsymbol{\Pi})\cdot(\boldsymbol{I}-\boldsymbol{\Pi})=\boldsymbol{I}-\boldsymbol{\Pi}\,,\ \ (\boldsymbol{I}-\boldsymbol{\Pi})\cdot\boldsymbol{\Pi}=\boldsymbol{0}\,,$$

one can easily find the explicit formula for the Fourier transform $\boldsymbol{g}^{(q)}(\mathbf{k})$:

$$\begin{aligned}\tilde{g}_{ij}^{(q)}(\mathbf{q}) &= \left[\frac{1}{{c_{L_q}}^2 q^2-\omega^2}\,\Pi_{ij}+\frac{1}{{c_{T_q}}^2 q^2-\omega^2}(\delta_{ij}-\Pi_{ij})\right]\\ &= \left(\frac{1}{{c_{L_q}}^2 q^2-\omega^2}-\frac{1}{{c_{T_q}}^2 q^2-\omega^2}\right)\Pi_{ij}+\frac{1}{{c_{T_q}}^2 q^2-\omega^2}\,\delta_{ij}\\ &= \frac{1}{\omega^2}\left(\frac{1}{q^2-{k_{L_q}}^2}-\frac{1}{q^2-{k_{T_q}}^2}\right)q_i q_j+\frac{1}{{c_{T_q}}^2}\frac{1}{q^2-{k_{T_q}}^2}\,\delta_{ij}\,,\end{aligned} \tag{S84}$$

where $k_{T_q}\equiv\omega/c_{T_q}$ and $k_{L_q}\equiv\omega/c_{L_q}$. Using the relation between the Fourier transform of derivatives, we can write

$$\tilde{g}_{ij}^{(q)}(\mathbf{q}) = -\frac{1}{\omega^2}\text{F.T.}\left\{\frac{\partial^2}{\partial x_i\partial x_j}\text{F.T.}^{-1}\left[\frac{1}{q^2-{k_{L_q}}^2}-\frac{1}{q^2-{k_{T_q}}^2}\right]\right\}+\frac{1}{{c_{T_q}}^2}\frac{1}{q^2-{k_{T_q}}^2}\delta_{ij}, \tag{S85}$$

where F.T. and F.T.$^{-1}$ represent the Fourier and inverse Fourier transforms, respectively.

We note that the inverse Fourier transform of $(k^2-{k_{L_q}}^2)^{-1}$ corresponds to the Green function $g_H(\mathbf{r};k_{L_q})$ of the Helmholtz equation with a wavenumber $k_{L_q}$ in infinite space $\mathbb{R}^d$ given in

$$\frac{\partial^2 g_H(\mathbf{r};k_{L_q})}{\partial x_i^2}+{k_{L_q}}^2\,g_H(\mathbf{r};k_{L_q}) = -\,\delta(\mathbf{r})\,, \tag{S86}$$

where $\mathbf{r}\equiv\mathbf{x}-\mathbf{x}'$. In direct space, an explicit formula for this Green function is well-known:

$$g_H(\mathbf{r};k) = \frac{i}{4}\left(\frac{k}{2\pi|\mathbf{r}|}\right)^{d/2-1}\mathcal{H}^{(1)}_{d/2-1}(k|\mathbf{r}|)\,, \tag{S87}$$

which reduces for $d=1,3$ as

$$g_H(\mathbf{r};k) = \begin{cases}\frac{ie^{ik|r|}}{2|k|}, & d=1\\ \frac{e^{ik|\mathbf{r}|}}{4\pi|\mathbf{r}|}, & d=3\end{cases}. \tag{S88}$$

Using (S87) and the following identities

$$\frac{\partial r^{-\alpha}}{\partial x_i} = -\alpha\hat{\mathbf{r}}_i r^{-\alpha-1}, \tag{S89}$$

$$\frac{\partial\hat{\mathbf{r}}_j}{\partial x_j} = \frac{1}{r}(\delta_{ij}-\hat{\mathbf{r}}_i\hat{\mathbf{r}}_j), \tag{S90}$$

one can explicitly writes out the dyadic Green function as follows:

$$g_{ij}^{(q)}(\mathbf{x},\mathbf{x}') = -\frac{1}{\omega^2}\frac{\partial^2}{\partial x_i\partial x_j}\left[g_H(\mathbf{r};k_{L_q})-g_H(\mathbf{r};k_{T_q})\right]+\frac{{k_{T_q}}^2}{\omega^2}\,g_H(\mathbf{r};k_{T_q})\,\delta_{ij} \tag{S91}$$

$$\begin{aligned}=&\frac{1}{\omega^2}\left[g_H''(r;k_{T_q})-g_H''(r;k_{L_q})-\frac{1}{r}\left(g_H'(r;k_{T_q})-g_H'(r;k_{L_q})\right)\right]\hat{\mathbf{r}}_i\hat{\mathbf{r}}_j\\ &+\frac{1}{\omega^2}\left[\frac{1}{r}\left(g_H'(r;k_{T_q})-g_H'(r;k_{L_q})\right)+{k_{T_q}}^2\,g_H(r;k_{T_q})\right]\delta_{ij}\end{aligned} \tag{S92}$$

$$= A_d(r)\,\hat{\mathbf{r}}_i\hat{\mathbf{r}}_j+B_d(r)\,\delta_{ij}, \tag{S93}$$

where the prime symbol ($'$) denotes the derivative with respect to $r$, and

$$A_d(r) = \frac{-i\pi}{2\omega^2(2\pi)^{d/2}r^d}\left[(k_{L_q}r)^{d/2+1}\,\mathcal{H}^{(1)}_{d/2+1}(k_{L_q}r)-(k_{T_q}r)^{d/2+1}\,\mathcal{H}^{(1)}_{d/2+1}(k_{T_q}r)\right], \tag{S94}$$

$$B_d(r) = \frac{i\pi}{2\omega^2(2\pi)^{d/2}r^d}\left[\left(k_{L_q}r\right)^{d/2}\mathcal{H}^{(1)}_{d/2}(k_{L_q}r)-\left(k_{T_q}r\right)^{d/2}\mathcal{H}^{(1)}_{d/2}(k_{T_q}r)+(k_{T_q}r)^{d/2+1}\,\mathcal{H}^{(1)}_{d/2-1}(k_{T_q}r)\right]. \tag{S95}$$

### B. Fourth-Rank Green Function $\boldsymbol{G}^{(q)}(\mathbf{r})$

We derive the fourth-rank Green function employed in (S13). To do so, we first need to derive the integral equation (S13) from (S11).

$$\begin{aligned}\epsilon_{ij}(\mathbf{x}) - (\epsilon_0)_{ij}(\mathbf{x}) &= \frac{1}{2}\left[\frac{\partial\,\check{u}_i(\mathbf{x})}{\partial x_j} + \frac{\partial\,\check{u}_j(\mathbf{x})}{\partial x_i}\right] = \frac{1}{2}\int_\epsilon \mathrm{d}\mathbf{x}'\left(\frac{\partial\, g^{(q)}_{ik}}{\partial x_j} + \frac{\partial\, g^{(q)}_{jk}}{\partial x_i}\right)\frac{\partial\, P_{kl}(\mathbf{x}')}{\partial x'_l} \\ &= \frac{1}{2}\int_\epsilon \mathrm{d}\mathbf{x}'\,\frac{\partial}{\partial x'_l}\left[\left(\frac{\partial g^{(q)}_{ik}}{\partial x_j} + \frac{\partial g^{(q)}_{jk}}{\partial x_i}\right)P_{kl}(\mathbf{x}')\right] - \frac{1}{2}\int_\epsilon \mathrm{d}\mathbf{x}'\,\frac{\partial}{\partial x'_l}\left(\frac{\partial g^{(q)}_{ik}}{\partial x_j} + \frac{\partial g^{(q)}_{jk}}{\partial x_j}\right)P_{kl}(\mathbf{x}')\,,\end{aligned} \tag{S96}$$

where we have used integration by parts to remove the divergence applied to the polarization tensor. Applying the divergence theorem to the first integral in (S96) yields

$$\epsilon_{ij}(\mathbf{x}) - (\epsilon_0)_{ij}(\mathbf{x}) = \frac{1}{2}\oint_\epsilon \mathrm{d}a'\,\hat{\mathbf{r}}_l\left[\left(\frac{\partial g^{(q)}_{ik}}{\partial x_j} + \frac{\partial g^{(q)}_{jk}}{\partial x_i}\right)P_{kl}(\mathbf{x}')\right] - \frac{1}{2}\int_\epsilon \mathrm{d}\mathbf{x}'\,\frac{\partial}{\partial x'_l}\left(\frac{\partial g^{(q)}_{ik}}{\partial x_j} + \frac{\partial g^{(q)}_{jk}}{\partial x_j}\right)P_{kl}(\mathbf{x}')\,, \tag{S97}$$

where $\oint_\epsilon \mathrm{d}a'\,\hat{\mathbf{r}}_l$ denotes the surface integral over the exclusion-region boundary.

Use of (S93), (S89), and (S90) gives an expression for the integrand in the first integral (S97):

$$\begin{aligned}\left(\frac{\partial g^{(q)}_{ik}}{\partial x_j} + \frac{\partial g^{(q)}_{jk}}{\partial x_i}\right) &= \left[(\hat{\mathbf{r}}_i\delta_{jk} + \hat{\mathbf{r}}_j\delta_{ik} + 2\hat{\mathbf{r}}_k\delta_{ij})\frac{A_d(r)}{r} + (\hat{\mathbf{r}}_j\delta_{ik} + \hat{\mathbf{r}}_i\delta_{jk})B'_d(r)\right] \\ &\quad + 2\hat{\mathbf{r}}_i\hat{\mathbf{r}}_k\hat{\mathbf{r}}_j\left[A'_d(r) - \frac{2}{r}A_d(r)\right].\end{aligned} \tag{S98}$$

Thus, for a spherical exclusion-region, the first integral in (S97) is written as

$$\begin{aligned}&\frac{1}{2}\lim_{r\to 0^+} r^{d-1}\left\{\frac{A_d(r)}{r}\oint_r d\Omega_d\,\hat{\mathbf{r}}_l(\hat{\mathbf{r}}_i\delta_{jk} + \hat{\mathbf{r}}_j\delta_{ik} + 2\hat{\mathbf{r}}_k\delta_{ij})\,P_{kl}(\mathbf{x}') + B'_d(r)\oint_r d\Omega_d\,\hat{\mathbf{r}}_l(\hat{\mathbf{r}}_j\delta_{ik} + \hat{\mathbf{r}}_i\delta_{jk})\,P_{kl}(\mathbf{x}')\right. \\ &\left.\quad + 2\left[A'_d(r) - \frac{2}{r}A_d(r)\right]\oint_r d\Omega_d\,\hat{\mathbf{r}}_i\hat{\mathbf{r}}_j\hat{\mathbf{r}}_k\hat{\mathbf{r}}_l\,P_{kl}(\mathbf{x}')\right\}\end{aligned} \tag{S99}$$

$$\begin{aligned}=&\frac{1}{2}\left\{\lim_{r\to 0^+}\left[r^{d-2}A_d(r)\right]\lim_{r\to 0^+}\oint_r d\Omega_d\,\hat{\mathbf{r}}_l(\hat{\mathbf{r}}_i\delta_{jk} + \hat{\mathbf{r}}_j\delta_{ik} + 2\hat{\mathbf{r}}_k\delta_{ij})\,P_{kl}(\mathbf{x}')\right. \\ &+ \lim_{r\to 0^+}\left[r^{d-1}B'_d(r)\right]\lim_{r\to 0^+}\oint_r d\Omega_d\,\hat{\mathbf{r}}_l(\hat{\mathbf{r}}_j\delta_{ik} + \hat{\mathbf{r}}_i\delta_{jk})\,P_{kl}(\mathbf{x}') \\ &\left.+ 2\lim_{r\to 0^+} r^{d-1}\left[A'_d(r) - \frac{2}{r}A_d(r)\right]\lim_{r\to 0^+}\oint_r d\Omega_d\,\hat{\mathbf{r}}_i\hat{\mathbf{r}}_j\hat{\mathbf{r}}_k\hat{\mathbf{r}}_l\,P_{kl}(\mathbf{x}')\right\}\end{aligned} \tag{S100}$$

$$= -\frac{1}{(2+d)d}\left(\frac{2}{{c_L}^2} - \frac{d}{{c_T}^2}\right)P_{ij}(\mathbf{x}) - \frac{1}{(2+d)d}\left(\frac{1}{{c_L}^2} - \frac{1}{{c_T}^2}\right)P_{kk}(\mathbf{x})\,\delta_{ij} \tag{S101}$$

$$= -\left[\frac{1}{d{c_L}^2}(\Lambda_h)_{ijkl} + \frac{1}{d+2}\left(\frac{2}{d{c_L}^2} + \frac{1}{{c_T}^2}\right)(\Lambda_s)_{ijkl}\right]P_{kl}(\mathbf{x}) \equiv -D^{(q)}_{ijkl}\,P_{kl}(\mathbf{x})\,, \tag{S102}$$

where $A_d(r)$ and $B_d(r)$ are given in (S94) and (S95), respectively, and we have used expressions in Sec. III E.

The second term in (S97) is obtained by using $-\frac{\partial}{\partial x'_l} \to \frac{\partial}{\partial x_l}$ and then using the fact that $P_{kl}$ is a symmetric tensor:

$$\begin{aligned}&-\frac{1}{2}\int_\epsilon \mathrm{d}\mathbf{x}'\,\frac{\partial}{\partial x'_l}\left(\frac{\partial g^{(q)}_{ik}}{\partial x_j} + \frac{\partial g^{(q)}_{jk}}{\partial x_j}\right)P_{kl}(\mathbf{x}') = \frac{1}{2}\int_\epsilon \mathrm{d}\mathbf{x}'\,\frac{\partial}{\partial x_l}\left(\frac{\partial g^{(q)}_{ik}}{\partial x_j} + \frac{\partial g^{(q)}_{jk}}{\partial x_j}\right)P_{kl}(\mathbf{x}') \\ &= \int_\epsilon \frac{1}{4}\left[\frac{\partial^2 g^{(q)}_{ik}}{\partial x_j\partial x_l} + \frac{\partial^2 g^{(q)}_{jk}}{\partial x_i\partial x_l} + \frac{\partial^2 g^{(q)}_{il}}{\partial x_j\partial x_k} + \frac{\partial^2 g^{(q)}_{jl}}{\partial x_i\partial x_k}\right]P_{kl}(\mathbf{x}')\,\mathrm{d}\mathbf{x}' \equiv \int_\epsilon H^{(q)}_{ijkl}(\mathbf{x}-\mathbf{x}')\,P_{kl}(\mathbf{x}')\,\mathrm{d}\mathbf{x}'\,.\end{aligned} \tag{S103}$$

Thus, the fourth-rank tensor $\boldsymbol{H}^{(q)}(\mathbf{r})$ meets (S17). Combination of (S102) and (S103) results in (S14).

**Remarks:**

1. The constant $\boldsymbol{D}^{(q)}$ also can be computed by using (S36) in the limit of $|\mathbf{q}| \to 0^+$.

## III. USEFUL IDENTITIES

In this section, we list some useful identities that are frequently used in this paper.

### A. Recurrence Relation

Here, we present a useful recurrence relation associated with Bessel functions as well as Hankel functions that is heavily used to simplify formulas in Sec. I C. Specifically, for all $\nu > 0$,

$$2\nu\, Z_\nu(x) = x\, Z_{\nu-1}(x) + x\, Z_{\nu+1}(x)\,, \tag{S104}$$

where $Z_\nu(x)$ corresponds to Bessel function of the first kind $J_\nu(x)$, Bessel function of the second kind $Y_\nu(x)$, and Hankel function of the first kind $\mathcal{H}_\nu^{(1)}(x)$. From this recurrence relation, one can also obtain the following identity

$$\frac{3}{d(d+2)} x^2\, Z_{d/2+3}(x) + \frac{6}{d} x\, Z_{d/2+2}(x) + 3\, Z_{d/2+1}(x) = \frac{3}{d(d+2)} x^2\, Z_{d/2-1}(x)\,.$$

### B. Properties of Projection Tensors

Here, we briefly discuss important properties of the hydrostatic projection tensor $\mathbf{\Lambda}_h$ and the shear projection tensor $\mathbf{\Lambda}_s$; see the main text for definitions. While the former $\mathbf{\Lambda}_h$ projects onto fields that are isotropic everywhere, whereas the latter $\mathbf{\Lambda}_s$ projects onto fields that are trace-free. These two tensors are useful due to the following identities:

$$\mathbf{\Lambda}_h + \mathbf{\Lambda}_s = \boldsymbol{I}\,, \tag{S105}$$

$$\mathbf{\Lambda}_h : \mathbf{\Lambda}_s = \mathbf{\Lambda}_s : \mathbf{\Lambda}_h = 0, \tag{S106}$$

$$\mathbf{\Lambda}_h : \mathbf{\Lambda}_h = \mathbf{\Lambda}_h\,, \tag{S107}$$

$$\mathbf{\Lambda}_s : \mathbf{\Lambda}_s = \mathbf{\Lambda}_s\,, \tag{S108}$$

$$\mathbf{\Lambda}_h \,\vdots\, \mathbf{\Lambda}_h = \mathbf{\Lambda}_h \,\vdots\, \boldsymbol{I} = 1, \tag{S109}$$

$$\mathbf{\Lambda}_s \,\vdots\, \mathbf{\Lambda}_s = \mathbf{\Lambda}_s \,\vdots\, \boldsymbol{I} = \frac{(d-1)(d+2)}{2}, \tag{S110}$$

where the symmetric fourth-order identity tensor $\boldsymbol{I}$ is defined in a component form as

$$I_{ijkl} \equiv \frac{1}{2}(\delta_{ik}\,\delta_{jl} + \delta_{il}\,\delta_{jk}). \tag{S111}$$

### C. Properties of $\boldsymbol{H}^{(q)}(\mathbf{r})$

We list traces of the fourth-rank tensor $\boldsymbol{H}^{(q)}(\mathbf{r})$ given in (S26):

$$H^{(q)}_{iikl}(\mathbf{r}) = \frac{i\pi}{2(2\pi)^{d/2}} \frac{1}{\omega^2 r^{d+2}} {r_L}^{d/2+2} \left[ -\mathcal{H}^{(1)}_{d/2}(r_L)\,\delta_{kl} + r_L\,\mathcal{H}^{(1)}_{d/2+1}(r_L)\,\hat{r}_k\,\hat{r}_l \right], \tag{S112}$$

$$H^{(q)}_{iijj}(\mathbf{r}) = \frac{i\pi}{2(2\pi)^{d/2}} \frac{1}{\omega^2 r^{d+2}} {r_L}^{d/2+2} \left[ -r_L\,\mathcal{H}^{(1)}_{d/2-1}(r_L) \right], \tag{S113}$$

$$H^{(q)}_{ijij}(\mathbf{r}) = \frac{-i\pi}{2(2\pi)^{d/2}} \frac{1}{\omega^2 r^{d+2}} \left[ {r_L}^{d/2+3}\,\mathcal{H}^{(1)}_{d/2-1}(r_L) + \frac{d-1}{2} {r_T}^{d/2+3}\,\mathcal{H}^{(1)}_{d/2-1}(r_T) \right], \tag{S114}$$

where $r_L \equiv k_{L_q} r$ and $r_T \equiv k_{T_q} r$. In order to obtain these formulas, we apply the recurrence relations of Hankel functions given in (S104) to (S26).

### D. Tensor Contractions

Here, we present some formulas for the inner products (contractions) of tensors employed to express $\boldsymbol{H}^{(q)}(\mathbf{r})$ given in (S26). These formulas are heavily used in Sec. I C. For convenience, we defined the following two fourth-rank

tensors:

$$(T_a)_{ijkl}(\mathbf{r}) \equiv \delta_{ij}\hat{r}_k\hat{r}_l, \tag{S115}$$

$$(T_b)_{ijkl}(\mathbf{r}) \equiv \hat{r}_i\hat{r}_j\delta_{kl}. \tag{S116}$$

Double and quadruple contractions of two fourth-rank tensors are listed in Table S1 and S2, respectively.

TABLE S1. Double contractions of two four-rank tensors (i.e., $\boldsymbol{A} : \boldsymbol{B}$ or, equivalently, $A_{ijmn}\,B_{mnkl}$) in $\mathbb{R}^d$. Here, $\boldsymbol{T}_a$ and $\boldsymbol{T}_b$ are defined in (S115) and (S116), respectively.

| $\boldsymbol{A}$ \ $\boldsymbol{B}$ | $\boldsymbol{\Lambda}_h$ | $\boldsymbol{I}$ | $\boldsymbol{T}_1(\mathbf{r})$ | $\boldsymbol{T}_2(\mathbf{r})$ | $\boldsymbol{T}_3(\mathbf{r})$ |
|---|---|---|---|---|---|
| $\boldsymbol{\Lambda}_h$ | $\boldsymbol{\Lambda}_h$ | $\boldsymbol{\Lambda}_h$ | $\frac{1}{2}(\boldsymbol{\Lambda}_h + \boldsymbol{T}_a)$ | $\frac{1}{d}\boldsymbol{T}_a$ | $\frac{1}{d}\boldsymbol{T}_a$ |
| $\boldsymbol{I}$ | $\boldsymbol{\Lambda}_h$ | $\boldsymbol{I}$ | $\boldsymbol{T}_1$ | $\boldsymbol{T}_2$ | $\boldsymbol{T}_3$ |
| $\boldsymbol{T}_1(\mathbf{r})$ | $\frac{1}{2}(\boldsymbol{\Lambda}_h + \boldsymbol{T}_b)$ | $\boldsymbol{T}_1$ | $\frac{1}{2}\boldsymbol{T}_1 + \frac{d}{4}(\boldsymbol{\Lambda}_h + \boldsymbol{T}_3)$ | $\frac{1}{2}(\boldsymbol{T}_a + \boldsymbol{T}_3)$ | $\frac{1}{2}(\boldsymbol{T}_a + \boldsymbol{T}_3)$ |
| $\boldsymbol{T}_2(\mathbf{r})$ | $\frac{1}{d}\boldsymbol{T}_b$ | $\boldsymbol{T}_2$ | $\frac{1}{2}(\boldsymbol{T}_3 + \boldsymbol{T}_b)$ | $\frac{1}{2}(\boldsymbol{T}_2 + \boldsymbol{T}_3)$ | $\boldsymbol{T}_3$ |
| $\boldsymbol{T}_3(\mathbf{r})$ | $\frac{1}{d}\boldsymbol{T}_b$ | $\boldsymbol{T}_3$ | $\frac{1}{2}(\boldsymbol{T}_3 + \boldsymbol{T}_b)$ | $\boldsymbol{T}_3$ | $\boldsymbol{T}_3$ |

TABLE S2. Quadruple contractions of two fourth-rank tensors (i.e., $\boldsymbol{A} \vdots \boldsymbol{B}$ or, equivalently, $A_{ijkl}\,B_{ijkl}$) in $\mathbb{R}^d$.

| $\boldsymbol{A}$ \ $\boldsymbol{B}$ | $\boldsymbol{\Lambda}_h$ | $\boldsymbol{I}$ | $\boldsymbol{T}_1(\mathbf{r})$ | $\boldsymbol{T}_2(\mathbf{r})$ | $\boldsymbol{T}_3(\mathbf{r})$ | $\boldsymbol{T}_1(\mathbf{s})$ | $\boldsymbol{T}_2(\mathbf{s})$ | $\boldsymbol{T}_3(\mathbf{s})$ |
|---|---|---|---|---|---|---|---|---|
| $\boldsymbol{\Lambda}_h$ | 1 | 1 | 1 | $\frac{1}{d}$ | $\frac{1}{d}$ | 1 | $\frac{1}{d}$ | $\frac{1}{d}$ |
| $\boldsymbol{I}$ | 1 | $\frac{d(d+1)}{2}$ | 1 | $\frac{d+1}{2}$ | 1 | 1 | $\frac{d+1}{2}$ | 1 |
| $\boldsymbol{T}_1(\mathbf{r})$ | 1 | 1 | $\frac{d+1}{2}$ | 1 | 1 | $\frac{d(\hat{\mathbf{r}}\cdot\hat{\mathbf{s}})^2+1}{2}$ | $(\hat{\mathbf{r}}\cdot\hat{\mathbf{s}})^2$ | $(\hat{\mathbf{r}}\cdot\hat{\mathbf{s}})^2$ |
| $\boldsymbol{T}_2(\mathbf{r})$ | $\frac{1}{d}$ | $\frac{d+1}{2}$ | 1 | $\frac{d+3}{4}$ | 1 | $(\hat{\mathbf{r}}\cdot\hat{\mathbf{s}})^2$ | $\frac{(d+2)(\hat{\mathbf{r}}\cdot\hat{\mathbf{s}})^2+1}{4}$ | $(\hat{\mathbf{r}}\cdot\hat{\mathbf{s}})^2$ |
| $\boldsymbol{T}_3(\mathbf{r})$ | $\frac{1}{d}$ | 1 | 1 | 1 | 1 | $(\hat{\mathbf{r}}\cdot\hat{\mathbf{s}})^2$ | $(\hat{\mathbf{r}}\cdot\hat{\mathbf{s}})^2$ | $(\hat{\mathbf{r}}\cdot\hat{\mathbf{s}})^4$ |

### E. Integral over Orientations

It is useful to compute integrals of tensors over orientations in $\mathbb{R}^d$ for $d \geq 3$ when one computes $C_3^{(p)}(k_{L_q})$ and $D_3^{(p)}(k_{L_q})$ in Sec. I C 2. In $d$-dimensional spherical coordinates, the integral of a given tensor $\boldsymbol{U}(\hat{\mathbf{r}})$ over orientations can be written as

$$\oint \mathrm{d}\Omega\, \boldsymbol{U}(\hat{\mathbf{r}}) = \int_0^{\pi} \mathrm{d}\theta \sin^{d-2}(\theta) \underbrace{\left[\int_0^{2\pi} \mathrm{d}\phi \prod_{i=1}^{d-3} \int_0^{\pi} \mathrm{d}\theta_i \sin^i(\theta_i)\;\; \boldsymbol{U}(\hat{\mathbf{r}})\right]}_{\equiv \oint_{\hat{\mathbf{r}}\cdot\hat{\mathbf{e}}_d = \cos\theta} \mathrm{d}\Omega \boldsymbol{U}(\hat{\mathbf{r}})}, \tag{S117}$$

where $\hat{\mathbf{e}}_d$ is a unit vector along the rotation axis for the azimuthal angle $\phi$ (e.g., $\hat{\mathbf{z}}$ for $d = 3$), and $\oint_{\hat{\mathbf{r}}\cdot\hat{\mathbf{e}}_d=\cos\theta} \mathrm{d}\Omega\, \boldsymbol{U}(\hat{\mathbf{r}})$ [shortly, $\oint_\theta \mathrm{d}\Omega\, \boldsymbol{U}(\hat{\mathbf{r}})$] stands for an integral over a unit sphere satisfying the condition $\hat{\mathbf{r}} \cdot \hat{\mathbf{e}}_d = \cos\theta$.

Using an identity

$$\int_0^{\pi} d\theta \sin^n\theta = \sqrt{\pi}\frac{\Gamma((n+1)/2)}{\Gamma(n/2+1)}, \tag{S118}$$

one derives the following integrals:

$$\oint_\theta \mathrm{d}\Omega = \frac{2\sqrt{\pi}^{d-1}}{\Gamma((d-1)/2)} = \Omega_{d-1}, \tag{S119}$$

$$\oint_\theta \mathrm{d}\Omega\, \hat{\mathbf{r}}_i = \Omega_{d-1}\cos\theta(\hat{\mathbf{e}}_d)_i \tag{S120}$$

$$\oint_\theta \mathrm{d}\Omega\, \hat{\mathbf{r}}_i\hat{\mathbf{r}}_j = \frac{\Omega_{d-1}}{d-1}\big[\sin^2\theta\,\delta_{ij} + (d\cos^2\theta - 1)(\hat{\mathbf{e}}_d)_i(\hat{\mathbf{e}}_d)_j\big] \tag{S121}$$

$$\begin{aligned}\oint_\theta \mathrm{d}\Omega\, \hat{\mathbf{r}}_i\hat{\mathbf{r}}_j\hat{\mathbf{r}}_k\hat{\mathbf{r}}_l =& \frac{\Omega_{d-1}}{d-1}\Big\{\frac{1}{d+1}\sin^4\theta(\delta_{ij}\delta_{kl} + \delta_{ik}\delta_{jl} + \delta_{il}\delta_{jk}) \\ &+ \sin^2\theta\Big(1 - \frac{d+2}{d+1}\sin^2\theta\Big)[2\,\boldsymbol{T}_1(\hat{\mathbf{e}}_d) + 4\,\boldsymbol{T}_2(\hat{\mathbf{e}}_d)] \\ &+ \Big[(d-1)\cos^4\theta - 6\sin^2\theta + \frac{6d+9}{d+1}\sin^4\theta\Big]\,(\hat{\mathbf{e}}_d)_i(\hat{\mathbf{e}}_d)_j(\hat{\mathbf{e}}_d)_k(\hat{\mathbf{e}}_d)_l\Big\},\end{aligned} \tag{S122}$$

where $\Omega_d$ is the surface area of a unit sphere in $\mathbb{R}^d$. Use of (S119)-(S122) gives the orientation integrals of the following fourth-rank tensors $\boldsymbol{\Lambda}_h\,, \boldsymbol{I}\,, \boldsymbol{T}_1(\mathbf{r})\,, \boldsymbol{T}_2(\mathbf{r})\,, \boldsymbol{T}_3(\mathbf{r})$ as

$$\oint_\theta \mathrm{d}\Omega\,\boldsymbol{\Lambda}_h = \Omega_{d-1}\,\boldsymbol{\Lambda}_h\,, \qquad \oint_\theta \mathrm{d}\Omega\,\boldsymbol{I} = \Omega_{d-1}\,\boldsymbol{I} \tag{S123}$$

$$\oint_\theta \mathrm{d}\Omega\,\boldsymbol{T_1}(\mathbf{r}) = \frac{\Omega_{d-1}}{d-1}\big[d(1-\cos^2\theta)\,\boldsymbol{\Lambda}_h + (d\cos^2\theta - 1)\,\boldsymbol{T}_1(\hat{\mathbf{e}}_d)\big] \tag{S124}$$

$$\oint_\theta \mathrm{d}\Omega\,\boldsymbol{T}_2(\mathbf{r}) = \frac{\Omega_{d-1}}{d-1}\big[(1-\cos^2\theta)\,\boldsymbol{I} + (d\cos^2\theta - 1)\,\boldsymbol{T}_2(\hat{\mathbf{e}}_d)\big] \tag{S125}$$

$$\begin{aligned}\oint_\theta \mathrm{d}\Omega\,\boldsymbol{T}_3(\mathbf{r}) =& \frac{\Omega_{d-1}}{d-1}\Big\{\frac{1}{d+1}\sin^4\theta(d\,\boldsymbol{\Lambda}_h + 2\,\boldsymbol{I}) + \sin^2\theta\Big(1 - \frac{d+2}{d+1}\sin^2\theta\Big)[2\,\boldsymbol{T}_1(\hat{\mathbf{e}}_d) + 4\,\boldsymbol{T}_2(\hat{\mathbf{e}}_d)] \\ &+ \Big[(d-1)\cos^4\theta - 6\sin^2\theta + \frac{6d+9}{d+1}\sin^4\theta\Big]\,\boldsymbol{T}_3(\hat{\mathbf{e}}_d)\Big\}.\end{aligned} \tag{S126}$$

Substituting (S119)-(S122) into the orientation integral (S117) gives

$$\oint \mathrm{d}\Omega = \Omega_d, \tag{S127}$$

$$\oint \mathrm{d}\Omega\,\hat{\mathbf{r}}_i = 0, \tag{S128}$$

$$\oint \mathrm{d}\Omega\,\hat{\mathbf{r}}_i\hat{\mathbf{r}}_j = \frac{\Omega_d}{d}\delta_{ij}, \tag{S129}$$

$$\oint \mathrm{d}\Omega\,\hat{\mathbf{r}}_i\hat{\mathbf{r}}_j\hat{\mathbf{r}}_k\hat{\mathbf{r}}_l = \frac{\Omega_d}{d(d+2)}(\delta_{ij}\delta_{kl} + \delta_{ik}\delta_{jl} + \delta_{il}\delta_{jk}) = \frac{\Omega_d}{d+2}\Big([\Lambda_h]_{ijkl} + \frac{2}{d}[\boldsymbol{I}]_{ijkl}\Big) \tag{S130}$$

$$= \frac{\Omega_d}{d}\Big([\Lambda_h]_{ijkl} + \frac{2}{d+2}[\Lambda_s]_{ijkl}\Big). \tag{S131}$$

Use of (S129) and (S131) gives

$$\oint \mathrm{d}\Omega\,\boldsymbol{T}_1(\mathbf{r}) = \Omega_d\,\boldsymbol{\Lambda}_h\,, \tag{S132}$$

$$\oint \mathrm{d}\Omega\,\boldsymbol{T}_2(\mathbf{r}) = \frac{\Omega_d}{d}\,\boldsymbol{I} = \frac{\Omega_d}{d}(\boldsymbol{\Lambda}_h + \boldsymbol{\Lambda}_s), \tag{S133}$$

$$\oint \mathrm{d}\Omega\,\boldsymbol{T}_3(\mathbf{r}) = \frac{\Omega_d}{d+2}\Big(\boldsymbol{\Lambda_h} + \frac{2}{d}\,\boldsymbol{I}\Big) = \Omega_d\Big(\frac{1}{d}\,\boldsymbol{\Lambda}_h + \frac{2}{d(d+2)}\,\boldsymbol{\Lambda}_s\Big), \tag{S134}$$

$$\oint \mathrm{d}\Omega\,\boldsymbol{T}_a(\mathbf{r}) = \oint \mathrm{d}\Omega\,\boldsymbol{T}_b(\mathbf{r}) = \Omega_d\,\boldsymbol{\Lambda}_h\,, \tag{S135}$$

where $\boldsymbol{T}_a(\mathbf{r})$ and $\boldsymbol{T}_b(\mathbf{r})$ are defined in Eqs. (S115) and (S116), respectively.

## IV. EVALUATION OF THE ATTENUATION FUNCTIONS

It is difficult to compute the attenuation functions for general disordered media by using the expressions presented in the main text. Here, we present the expressions that are more convenient to compute. The reader is referred to Ref. [7] for derivations.

For the local attenuation function $\mathcal{F}(Q)$, it is useful to employ the following formulas:

$$\begin{aligned}\mathrm{Im}[\mathcal{F}(Q)] &= -\lim_{\epsilon\to0^+}\int_\epsilon^\infty \mathrm{d}r\, Q\,\chi_{_V}(r)\,(Qr)^{d/2}\,J_{d/2-1}(Qr)\\ &= -\frac{Q^d}{(2\pi)^{d/2}}\,\tilde{\chi}_{_V}(Q)\,, \end{aligned}\tag{S136}$$

$$\begin{aligned}\mathrm{Re}[\mathcal{F}(Q)] &= \lim_{\epsilon\to0^+}\int_\epsilon^\infty \mathrm{d}r\, Q\,\chi_{_V}(r)\,(Qr)^{d/2}\,Y_{d/2-1}(Qr)\\ &= -\frac{2Q^2}{\pi}\mathrm{p.v.}\int_0^\infty \mathrm{d}q\,\frac{1}{q(Q^2-q^2)}\,\mathrm{Im}[\mathcal{F}(q)], \end{aligned}\tag{S137}$$

where $J_\nu(x)$ is the Bessel function of the first kind of order $\nu$, $Y_\nu(x)$ is the Bessel function of the second kind of order $\nu$, and p.v. stands for the Cauchy principal value of an integral. Since the Cauchy principal value is difficult to handle in numerical integration, we reformulate (S137) as follows

$$\begin{aligned}\mathrm{Re}[\mathcal{F}(Q)] &\approx -\frac{2Q^2}{\pi}\left[\mathrm{p.v.}\int_0^M \frac{1}{q(Q^2-q^2)}\,\mathrm{Im}[\mathcal{F}(q)]\,\mathrm{d}q\right]\\ &= -\frac{2Q}{\pi}\left[\int_0^M \frac{\mathrm{Im}[\mathcal{F}(q)]}{(Q+q)q}\,\mathrm{d}q + \int_0^M \frac{\mathrm{Im}[\mathcal{F}(q)]-\mathrm{Im}[\mathcal{F}(Q)]}{Q^2-q^2}\,\mathrm{d}q\right], \end{aligned}\tag{S138}$$

where $M$ is the upper limit of numerical integral.

For the nonlocal attenuation function $F(Q)$ for statistically isotropic media, the following formulas are convenient to use:

$$\mathrm{Im}[F(Q)] = \begin{cases} -\frac{Q^2}{\pi^2}\int_0^{\pi/2}\tilde{\chi}_{_V}(2Q\cos\phi)\,\mathrm{d}\phi\,, & d=2\\ -\frac{Q}{2(2\pi)^{3/2}}\int_0^{2Q} q\,\tilde{\chi}_{_V}(q)\,\mathrm{d}q\,, & d=3 \end{cases}\tag{S139}$$

$$\mathrm{Re}[F(Q)] = -\frac{2Q^2}{\pi}\mathrm{p.v.}\int_0^\infty \mathrm{d}q\,\frac{1}{q(Q^2-q^2)}\,\mathrm{Im}[F(q)],\tag{S140}$$

where Eq. (S140) is valid for $d=2,3$. The nonlocal counterpart of (S138) is

$$\begin{aligned}\mathrm{Re}[F(Q)] &\approx -\frac{2Q^2}{\pi}\left[\mathrm{p.v.}\int_0^M \frac{1}{q(Q^2-q^2)}\,\mathrm{Im}[F(q)]\,\mathrm{d}q + \frac{\mathrm{Im}[F(M)]}{M}\int_M^\infty \frac{1}{Q^2-q^2}\,\mathrm{d}q\right]\\ &= -\frac{2Q}{\pi}\Big(\int_0^M \frac{\mathrm{Im}[F(q)]}{(Q+q)q}\,\mathrm{d}q + \int_0^M \frac{\mathrm{Im}[F(q)]-\mathrm{Im}[F(Q)]}{Q^2-q^2}\,\mathrm{d}q\\ &\quad + \frac{1}{2Q}\Big\{\mathrm{Im}[F(Q)] - \frac{Q}{M}\,\mathrm{Im}[F(M)]\Big\}\ln\left|\frac{M+Q}{M-Q}\right|\Big). \end{aligned}\tag{S141}$$

## V. SIMULATION DETAILS

Here we provide additional details about simulation procedures and values of the simulation parameters that we used. We list parameters employed to numerically generate sphere packings for computing the spectral density and the attenuation functions in Sec. V A. In Sec. V B, we describe the full-waveform simulations that we employed in the main text.

### A. Parameters for Numerically Generated Packings

We numerically generate packings in three dimensions for disordered stealthy hyperuniform packings and hyperuniform polydisperse packings to compute the spectral density $\tilde{\chi}_{_V}(Q)$. For each model, we generate $N_c$ different packings

of particle radius $a$, $N$ particles, and number density $\rho$ in a periodic fundamental cell. Here, we list these parameters as well as some other relevant parameters; see Table S3.

Stealthy hyperuniform packings are generated via the collective-coordinate optimization technique. For this model, a parameter $Q_{\mathrm{U}}$ defines the stealthy regions, and $\sigma$ represents the diameter of the repulsion region of each particle. For stealthy hyperuniform packings (or point patterns), it is useful to define the $\chi$ parameter, which the ratio of constrained degrees of freedom to total number of degrees of freedom [8, 9], i.e.,

$$\chi \equiv \frac{\mathcal{M}}{d(N-1)}. \tag{S142}$$

For $0 < \chi < 1/2$, they are highly degenerate and disordered, whereas for $1/2 < \chi < 1$ they crystallize [9].

TABLE S3. Parameters of sphere packings used to compute $\tilde{\chi}_V(Q)$. We generate realizations of disordered stealthy hyperuniform packings and hyperuniform polydisperse packings in three dimensions. For each model, $N_c$ is the number of distinct packings, $N$ particle number, $a$ is particle radius, $\rho$ is the number density, and $\phi_2$ is the packing fraction. For hyperuniform polydisperse packings, $a$ stands for the mean particle radius, i.e., $a \equiv [\phi_2/v_1(1)]^{1/d}$. Quantities $Q_{\mathrm{U}}$ and $\sigma$ are parameters used in the collective-coordinate optimization method; see Sec. III in the main text. The $\chi$ parameter is defined in Eq. (S142).

| Systems \Parameters | $N$ | $\rho$ | $N_c$ | $Q_{\mathrm{U}}a$ | $\sigma$ | $a$ | $\chi$ |
|---|---|---|---|---|---|---|---|
| 3D Stealthy hyperuniform packings ($\phi_2 = 0.25$) | 1000 | 1 | 300 | 1.5 | 0.8 | 0.3908 | 0.1582 |
| 3D Stealthy hyperuniform packings ($\phi_2 = 0.4$) | 1000 | 1 | 300 | 1.5 | 0.92 | 0.4571 | 0.1031 |
| 3D Hyperuniform ploydisperse packings ($\phi_2 = 0.25$) | 1000 | 1 | 300 | - | - | 0.3908 | - |

### B. Full-Waveform Simulations

We employ the dynamic extension of the fast-Fourier transform-based homogenization scheme devised for the purely static problem [10, 11]. We note that such dynamic extensions were first employed in Ref. [12]. The simulation results presented in the main text are obtained with setting the number of voxels in each side as $N_1 = N_2 = N_3 = 101$.

**Algorithm 1:** Fast-Fourier transform-based homogenization scheme for the effective dynamic bulk and shear moduli. The applied strain $\boldsymbol{\epsilon_0}$ and the associated wavevector $\mathbf{k}$ depend on the elastic moduli to compute:

$$
\begin{aligned}
(\epsilon_0)_{ij} =& \delta_{ij} \text{ with } \mathbf{k} = k_{L1}\,\hat{\mathbf{x}}, \quad \text{for } K_e \\
(\epsilon_0)_{ij} =& 1-\delta_{ij} \text{ with } \mathbf{k} = k_{T1}\,\hat{\mathbf{x}}, \quad \text{for } G_e.
\end{aligned}
$$

**Result:** $K_e$ or $G_e$ at a given frequency $\omega$

Set tolerance $\Delta = 10^{-9}$ and mass density $\rho_1 = \rho_2 = 1$.

Assign bulk modulus $K_i$ and shear modulus for phase $i$ $(= 1, 2)$.

Voxelize a two-phase medium in a periodic fundamental cell into $N_1 \times N_2 \times N_3$ voxels.

1. Set $m = 1$, $\Delta_{\text{div}} = 1$, $\boldsymbol{\epsilon}^{(0)}(\mathbf{x})\, e^{-i\mathbf{k}\cdot\mathbf{x}} = \boldsymbol{\epsilon}_0$, and $\boldsymbol{P}^{(0)}(\mathbf{x})\, e^{-i\mathbf{k}\cdot\mathbf{x}} = [\boldsymbol{C}(\mathbf{x}) - \boldsymbol{C}_1] : [\boldsymbol{\epsilon}^{(0)}(\mathbf{x})\, e^{-i\mathbf{k}\cdot\mathbf{x}}]$.

   **while** $\Delta_{\text{div}} > \Delta$ **do**

   i. $\tilde{\boldsymbol{P}}^{(m-1)}(\mathbf{q}+\mathbf{k}) = \text{FFT}\left[\boldsymbol{P}^{(m-1)}(\mathbf{x})\, e^{-i\mathbf{k}\cdot\mathbf{x}}\right]$.

   ii. Compute $\tilde{\boldsymbol{\sigma}}(\mathbf{q}+\mathbf{k}) = \boldsymbol{C}_1 : \tilde{\boldsymbol{\epsilon}}^{(m-1)}(\mathbf{q}+\mathbf{k}) + \tilde{\boldsymbol{P}}^{(m-1)}(\mathbf{q}+\mathbf{k})$ and the consequent error in wave equation:

   $$\Delta_{\text{div}} = \left\| \omega^2 \rho_1 \tilde{\epsilon}^{(m)}_{ij}(\mathbf{q}') - \frac{1}{2}\left[q'_i q'_l \tilde{\sigma}_{lj}(\mathbf{q}') + q'_j q'_l \tilde{\sigma}_{li}(\mathbf{q}')\right] \right\|,$$

   where $\mathbf{q}' \equiv \mathbf{q}+\mathbf{k}$, and for a second-rank tensor $\tilde{T}_{ij}(\mathbf{q})$, $\|\tilde{T}_{ij}(\mathbf{q})\| \equiv \left[\frac{1}{N_1N_2N_3}\sum_{\mathbf{q}}\sum_{i,j=1}^{3}\left|\tilde{T}_{ij}(\mathbf{q})\right|^2\right]^{1/2}$.

   **Stop if** $\Delta_{\text{div}} < \Delta$.

   iii. Using the Green function $\tilde{\boldsymbol{G}}^{(q)}(\mathbf{q})$ given in Eq. (S31), compute

   $$\tilde{\boldsymbol{\epsilon}}^{(m)}(\mathbf{q}+\mathbf{k}) = \begin{cases} N_1N_2N_3\,\boldsymbol{\epsilon}_0\,, & \mathbf{q} = \mathbf{0} \\ \tilde{\boldsymbol{G}}^{(q)}(\mathbf{q}+\mathbf{k}) : \tilde{\boldsymbol{P}}^{(m-1)}(\mathbf{q}+\mathbf{k})\,, & \text{otherwise} \end{cases}.$$

   iv. $\boldsymbol{\epsilon}^{(m)}(\mathbf{x})\, e^{-i\mathbf{k}\cdot\mathbf{x}} = \text{IFFT}[\tilde{\boldsymbol{\epsilon}}^{(m)}(\mathbf{q}+\mathbf{k})]$.

   v. Compute $\boldsymbol{P}^{(m)}(\mathbf{x})\, e^{-i\mathbf{k}\cdot\mathbf{x}} = [\boldsymbol{C}(\mathbf{x}) - \boldsymbol{C}_1] : \left[\boldsymbol{\epsilon}^{(m)}(\mathbf{x})\, e^{-i\mathbf{k}\cdot\mathbf{x}}\right]$.

   vi. Set $m \to m+1$.

   **end**

2. Compute the effective moduli:

   $$
   \begin{aligned}
   Ke =& \frac{\text{Tr}[\langle\boldsymbol{\sigma}\rangle]}{\text{Tr}[\langle\boldsymbol{\epsilon}\rangle]}, \\
   G_e =& \frac{1}{2}\frac{\sum_{i,j=1}^{d}\langle\sigma\rangle_{ij}}{\left[\sum_{i,j=1}^{d}\langle\epsilon\rangle_{ij}\right] - \text{Tr}[\langle\boldsymbol{\sigma}\rangle]},
   \end{aligned}
   $$

   where Tr[] denotes the trace, and

   $$
   \begin{aligned}
   \langle\boldsymbol{\sigma}\rangle =& \tilde{\boldsymbol{\sigma}}(\mathbf{k}) \\
   \langle\boldsymbol{\epsilon}\rangle =& \tilde{\boldsymbol{\epsilon}}^{(m)}(\mathbf{k})\,.
   \end{aligned}
   $$

---

[1] Rigorously speaking, this qualitative description is not accurate because elastic wave speeds generally vary with their polarizations (e.g., longitudinal or transverse).


[2] S. Torquato, "Effective stiffness tensor of composite media—I. Exact series expansions," J. Mech. Phys. Solids **45**, 1421–1448 (1997).

[3] S. Torquato, *Random Heterogeneous Materials: Microstructure and Macroscopic Properties*, Interdisciplinary Applied Mathematics (Springer Science & Business Media, 2002).

[4] W. F. Brown Jr., "Solid mixture permittivities," J. Chem. Phys. **23**, 1514–1517 (1955).

[5] S. Torquato, "Effective electrical conductivity of two-phase disordered composite media," J. Appl. Phys. **58**, 3790–3797 (1985).

[6] S. Torquato, "Exact Expression for the Effective Elastic Tensor of Disordered Composites," Phys. Rev. Lett. **79**, 681–684 (1997).
[7] S. Torquato and J. Kim, "Nonlocal Effective Electromagnetic Wave Characteristics of Composite Media: Beyond the Quasistatic Regime," arXiv:2007.00701 (2020), arXiv:2007.00701.
[8] S. Torquato, G. Zhang, and F. Stillinger, "Ensemble theory for stealthy hyperuniform disordered ground states," Phys. Rev. X **5**, 021020 (2015).
[9] G. Zhang, F. H. Stillinger, and S. Torquato, "Ground states of stealthy hyperuniform potentials: I. Entropically favored configurations," Phys. Rev. E **92**, 022119 (2015).
[10] H. Moulinec and P. Suquet, "A numerical method for computing the overall response of nonlinear composites with complex microstructure," Comput. Methods Appl. Mech. Engrg. **157**, 69–94 (1998).
[11] D. J. Eyre and G. W. Milton, "A fast numerical scheme for computing the response of composites using grid refinement," Eur. Phys. J. Appl. Phys. **6**, 41–47 (1999).
[12] J. Kim and S. Torquato, "Multifunctional Composites for Elastic and Electromagnetic Wave Propagation," Proc. Nat. Acad. Sci. U.S.A. **117**, 8764–8774 (2020).
